# Supplementary material for: Predictive model of surface adsorption in dissolution on transition metals and alloys
Source: arXiv:2108.11017 source file (2021-08-25)
Supplement: Supplementary file 1 [file Supplemental_Information.pdf]

# Supplemental Information

## Predictive model of surface adsorption in dissolution on transition metals and alloys

Bo Li, Wang Gao,* and Qing Jiang
Key Laboratory of Automobile Materials, Ministry of Education, Department of Materials Science and Engineering, Jilin University 130022, Changchun, China

**Table of Contents** **Page**


Note S1 .......... 4
Note S2 .......... 5
Note S3 .......... 6
Note S4 .......... 7
Note S5 .......... 8
Note S6 .......... 9
Note S7 .......... 10
FIG. S1 .......... 11
FIG. S2 .......... 12
FIG. S3 .......... 13
FIG. S4 .......... 14
FIG. S5 .......... 15
FIG. S6 .......... 16
FIG. S7 .......... 17
FIG. S8 .......... 18
FIG. S9 .......... 19
FIG. S10 .......... 20
FIG. S11 .......... 21
FIG. S12 .......... 22
FIG. S13 .......... 23
FIG. S14 .......... 24
FIG. S15 .......... 25
FIG. S16 .......... 26
FIG. S17 .......... 27
FIG. S18 .......... 28
FIG. S19 .......... 29
FIG. S20 .......... 30
FIG. S21 .......... 31
FIG. S22 .......... 32
FIG. S23 .......... 33
FIG. S24 .......... 34
FIG. S25 .......... 35
FIG. S26 .......... 36
FIG. S27 .......... 37
FIG. S28 .......... 38
FIG. S29 .......... 39
FIG. S30 .......... 40
FIG. S31 .......... 41
FIG. S32 .......... 42
FIG. S33 .......... 43

FIG. S34 ........ 44
FIG. S35 ........ 45
FIG. S36 ........ 46
FIG. S37 ........ 47
FIG. S38 ........ 48
FIG. S39 ........ 49
FIG. S40 ........ 50
Table S1 ........ 51
Table S2 ........ 52
Table S3 ........ 53
Table S4 ........ 54
Table S5 ........ 55
Table S6 ........ 56
Table S7 ........ 57
References ........ 58

**Note S1: Details of the adsorption systems and process in dissolution.**

We have considered the various adsorption systems including transition metals (TMs), near-surface alloys (NSAs), binary alloys (BAs), and high-entropy alloys (HEAs). TMs contain the close-packed surfaces (fcc(111), bcc(110) and hcp(0001) surfaces), (100), (110), and (211) surfaces. NSAs contain the (111) surface of Cu-based NSAs with the topmost layer being the alloying element, the (100) and (111) surfaces of Pt(Pd)-based NSAs with the subsurface layer being the alloying element, the (111) surface of Cu- and Ni-based CuNi NSAs with the different Cu/Ni ratios in the topmost and subsurface layers, the (111) surface of Au-based AuPd NSAs with the different ratio of Pd ensembles in the topmost layer, and the (111) surface of Pt-based NSAs with $A_xB_{3-x}/A_yB_{3-y}$ monolayers ($A_xB_{3-x}$($A_yB_{3-y}$) corresponds to the first (second) layer on Pt(111) host and the subscripts *x* and *y* denote the stoichiometry of the corresponding atoms). BAs contain the (100) and (111) surfaces of Ag-based AgM and Co-based CoM BAs with the stoichiometric ratio of 1 between the two components, the (111) surface of Ag-based $Ag_3M$ and Os-based $Os_3M$ BAs with the stoichiometric ratio of 3 between the two components, the (211) surface of AgAu, AgPd, IrRu, and PtRh BAs, and the (111) surface of La-series $Pt_5M$ BAs with the stoichiometric ratio of 5 between the two components and the topmost layer being the Pt element. HEAs contain the (100), (110), (111), (211) and (532) surfaces of Ru(Cu)RhIrPdPt-based HEAs (see the schematic atomic structures of Fig. S1).

The adsorption process covers several steps as the dissolution proceeds, which is shown in Fig. S2 for TM(111) surface. For NSAs, the dissolution process is the same as that for TMs since the surface of NSAs consists of only one element (Fig. S3a-d). For BAs, the practical dissolution order is adopted for adsorption, namely, the dissolution proceeds along the line composed of the same element shown in Fig. S3e-h. For HEAs, the similar steps as TMs are adopted for simulating the surface adsorption in dissolution, which don't correspond to the practical dissolution order of the different components (Fig. S4). Nevertheless, our calculations for HEAs are representative enough to consider all the possible cases of adsorption in dissolution (including the practical dissolution order), by substituting the adsorption site with the different elements in the adsorption-site effect of alloying.

## Note S2: Calculation details.

In this study, we performed the DFT-calculations with the Vienna Ab initio Simulation Package (VASP) [1] by using the projector augmented wavefunctions (PAW) [2] and Perdew−Burke−Ernzerhof (PBE) [3] and Perdew-Wang-91 (PW91) [4] functionals. At least four-layer slabs were built for modeling the TM and alloy surfaces, where the top two layers were fully relaxed and the rest layers were fixed in their optimized lattice. A vacuum of 20 Å was adopted to separate the adjacent slabs. The plane-wave cutoff energy of 500 eV was adopted for geometry optimization. The adsorption system was modeled at low coverage with the (2 × 2) supercell for (100) and (111) surfaces of TMs, NSAs, and BAs, and the (1 × 3) supercell for (211) surface of TMs. Note that we also adopted the (3 × 3) supercell for (111) surface of TMs. For HEAs, the larger unit cells were built than other systems to model the random composition and chemical ordering of HEAs, which were (4 × 4) supercell for (100), (110) and (111) surfaces, (2 × 4) supercell for (211) surface, and (2 × 2) supercell for (532) surface. We also discussed the coverage-dependent effects of adsorption energy as shown in Note S3. Therefore, the 6 × 6 × 1 Monkhorst-Pack k-point sampling mesh was used for TMs, NSAs, and BAs except for the TM(111) surface with (3 × 3) supercell (the 4 × 4 × 1 mesh was used for TM(111) surface with (3 × 3) supercell), and the 2 × 2 × 1 mesh was used for HEAs after careful tests (the step size was less than 0.03 1/Å for geometry optimization on all considered systems), which had also been proved to be sufficiently accurate for calculating the adsorption energy in Refs. [5,6]. For the electronic structure calculations, the k-point sampling meshes were 10 × 10 × 1 for TMs and 6 × 6 × 1 for HEAs. The calculations of transition states for $CH_2 \rightarrow CH + H$ on HEAs were performed with the same parameters as those for geometry optimization. The conjugate gradient algorithm was utilized with a convergence threshold of 0.02 eV/Å in Hellmann-Feynman force on each atom. Fermi smearing function was used with a smearing width of 0.1 eV to facilitate the convergence. Note that the PBE and PW91 functionals were adopted in our calculations while the cited calculations in Refs. [5–17] adopted the PBE, revised PBE (RPBE) [18], PW91, Bayesian error estimation functional with van der Waals correlation (BEEF-vdW) [19] and PBE-vdW [20] functionals.

The adsorption energy in this study was defined as,

$$E_{\mathrm{ad}} = E_{\mathrm{ref/sub}} - E_{\mathrm{sub}} - E_{\mathrm{ref}} \quad (1)$$

where $E_{\mathrm{ref/sub}}$, $E_{\mathrm{sub}}$, and $E_{\mathrm{ref}}$ represent the total energies of the adsorbed system, the clean substrate, and the gas reference of adsorbates. For consistency, we have unified the gas references from the different literatures [5–15]: CO, $H_2O$ and $H_2$ for $CH_x$ ($x$ = 1-3), $CCH_3$ and CO; $CH_4$ and $H_2$ for C; $N_2$ and $H_2$ for $NH_x$ ($x$ = 0-2); and $H_2O$ and $H_2$ for OH.

## Note S3: The coverage effects of adsorption.

To understand the coverage-dependent effects of adsorption energy, Fig. S15 shows the adsorption energy of C, CH, and N at the fcc and hcp sites of TM(111) surface with (1 × 1), (2 × 1), (2 × 2), and (4 × 4) supercells [8]. Encouragingly, all the adsorption energies at the different coverages can be well described by the electronic descriptor $\psi_0$ and geometric descriptor $\overline{CN}$ with the fitted mean absolute error (MAE) of 0.15 eV, smaller than the approximate error of (semi-)local functionals, ±0.2 eV. Namely, our scheme can be also used to capture the coverage effects of adsorption energy. However, the prefactors $\mu_1$ and $\mu_2$ and the parameter $\theta$ in Eq. (2) in the main text vary with coverage, which can be explained by the bonding properties of adsorbates and substrates. At low coverage, the interactions between adsorbates are negligible, therefore, the fitted prefactors $\mu_1$ and $\mu_2$ and the parameter $\theta$ are consistent with the prediction by Eq. (2) in the main text. Namely, Eqs. (2-4) in the main text is effective for the adsorption at low coverage, which has also been identified by our additional calculations for the adsorption energy of $CH_2$ and $NH_2$ at (3 × 3) supercell of TMs in dissolution (see Figs. S11 and S14a). At high coverage, the coverage effects generate the interactions between adsorbates, which change the bonding properties of adsorbate $X$ in Eq. (2) in the main text and thus lead to the different prefactors $\mu_1$ and $\mu_2$. On the other hand, the interactions between adsorbates also change the coupling strength between the *sp* states of substrates and the states of adsorbates, thus changing the parameter $\theta$.

Note that the bond-order conservation framework [21], the *d*-band based model [8,22], the mean-field coverage with linear and higher-order parametrizations [23], and the lattice gas Hamiltonian approach [24–26] have provided helpful insights about the coverage effects of adsorption energy. For instance, the *d*-band width/center and partial charges of the low-coverage adsorbed systems have been used as the descriptors for the high-coverage adsorption [8]. In contrast, our scheme is different from these models by directly including the effect of adsorbate-adsorbate interactions on the adsorbate valence, and thus is also convenient for applications.

## Note S4: The origin of the prefactors $\mu_1$ and $\mu_2$ in Eq. (2) in the main text.

Eq. (2) in the main text indicates that the prefactors $\mu_1$ and $\mu_2$ are determined by the valence of adsorbates, which can be deduced and rationalized from effective medium theory (EMT) and bond-order conservation framework [27]. In EMT, the inhomogeneous environment of the host is replaced by the homogeneous electron gas, thereby simplifying the calculations of the energies of the adsorption system [28]. It has been demonstrated that the first-order approximation of EMT is essential for describing the adsorption of atoms that are not particularly polarizable such as hydrogen and oxygen [28]. Note that the zero-order approximation of EMT has been derived by Nørskov *et al* [29] with the relation $E^{(0)} \propto \frac{(X_m - X)n_0}{X_m}$ ($n_0$ corresponds to the homogeneous electron density). For the first-order approximation, we adopt a simple perturbation effect induced by the adsorbed atom to the electron density as $\Delta n = \frac{n_0}{X_m + 1}$ ("1" stems from that the change of the bond number of adsorbate towards adsorption is most likely an integer and one). By substituting $n_0$ with $\Delta n$ in the zero-order term, the first-order term of EMT obeys that:

$$E^{(1)} \propto \frac{(X_m - X)n_0}{X_m(X_m + 1)} = (X_m - X)n_0\left(\frac{1}{X_m} - \frac{1}{X_m + 1}\right) \quad (2)$$

Combining the zero-order and the first-order terms of EMT, the adsorption energy of adsorbates that are not particularly polarizable obeys the relation as,

$$E_{ad} = E^{(0)} - E^{(1)} \propto \frac{(X_m - X)n_0}{X_m + 1} \quad (3)$$

This exactly corresponds to the prefactor $\mu_1$ in Eq. (2) in the main text. The prefactor $\mu_2$ in Eq. (2) in the main text, $\frac{X+1}{X_m+1}$, can be rationalized by the bond-order conservation framework. The adsorption energy is proportional to the coordination number of surface sites, namely the saturated-bond number of surface sites, which should also hold from the point of view of adsorbates. Thus, the adsorption energy is proportional to the bond number of adsorbates, corresponding to the prefactor $\frac{X+1}{X_m+1}$.

Table I shows that the DFT-calculated prefactors $\mu_1$ and $\mu_2$ for the adsorption energy on TMs, NSAs, BAs, and HEAs are in good agreement with the predictions by Eq. (2) in the main text, indicating that the prefactors $\mu_1$ and $\mu_2$ are solely determined by the adsorbates while are independent of the types of substrates. This demonstrates that the EMT and bond-order conservation framework are general in describing the adsorption on TMs and alloys. Namely, alloys, regardless of various components, exhibit a unified behavior for surface adsorption due to the alloying effects, which can be well described by the homogeneous-electron-gas model like EMT.

## Note S5: The environment effect of alloying on the adsorption energy.

Fig. 2c and d in the main text and Fig. S22 demonstrate that the adsorption energy of $CH_x$ ($x$=0-3), $NH_x$ ($x$=0-2), CO, OH, F and Cl on Ag-based BAs, Pt(Pd)-based NSAs and Ru(Cu)RhIrPdPt-based HEAs in the environment effect of alloying (namely fixing the chemical composition of adsorption sites and altering surrounding environments) also follows the linear relations in the adsorption-site effect of alloying, although the prefactors $k_1$ and $k_2$ in the $D_{ad}$ of Eq. (4) in the main text are different from that in the adsorption-site effect of alloying upon adsorbing on the different elements (Table S4). Notably, our scheme performs well in describing the adsorption of OH, F and Cl on NSAs that cannot be accurately described by the $d$-band model, not to mention the adsorption energy on BAs and HEAs that can hardly be described by the $d$-band model. Since $k_1$ and $k_2$ reflect the electronic localization of alloys in adsorption, one can estimate the localization of the different alloying elements in determining the adsorption energy according to the ratio of these two prefactors. For the $CH_2$ adsorption on HEAs, the ratio $k_1/k_2$ is 0.67 for dissolving Ru element, 0.80 for dissolving Ir element, 0.91 for dissolving Pt element, 2.65 for dissolving Pd element, and 12.17 for dissolving Rh element (see Table S4). Therefore, the localization of RuRhIrPdPt HEAs in adsorbing $CH_2$ during the dissolution obeys the order of Ru > Ir > Pt > Pd > Rh. Similarly, Cu is more local than Ru in adsorbing CO on Ru(Cu)RhIrPdPt-based HEAs (see Table S4).

**Note S6: The adsorption at the different sites of TMs and alloys with the different methods.**

In this study, we have considered the adsorption energy of various adsorbates at the top, bridge, fcc, hcp and four-fold sites of (100), (110), (111), and (211) surfaces of TMs, the top and fcc sites of (100) and (111) surfaces of NSAs, the top, bridge, fcc, hcp and four-fold sites of (100), (111) and (211) surfaces of BAs, and the top and bridge sites of (100), (110), (111), (211) and (532) surfaces of HEAs. Encouragingly, all these adsorption energies at the various sites of TMs and alloys can be well described by the electronic and geometric descriptors $D_{ad}$ and $\overline{CN}$, which demonstrates the universality of our scheme (see Fig. 2 in the main text and Figs. S13-S15, S20-S26) [5–15]. Note that our scheme can capture the adsorption energy of OH at the bridge site of HEAs in both the adsorption-site and environment effects of alloying by fixing one or two surrounding atoms of adsorption sites (see Figs. S25 and S26) [5]. For instance, the composition of one nearest-neighbor atom of adsorption sites is fixed as the Pd element to decrease the degree of freedom for the OH adsorption at the random bridge sites of HEA(211) surface (Fig. S26a). Apparently, the adsorption energy of OH at the bridge sites of HEAs with the different fixed surrounding atoms exhibits a universal linear relation with $D_{ad}$ and $\overline{CN}$.

Encouragingly, the prefactors of the $D_{ad}$ and $\overline{CN}$ terms $\mu_1$ and $\mu_2$ for the adsorption energy at the different adsorption sites of TMs, NSAs, BAs, and HEAs are all determined by the bonding characters $X_m$ and $X$ of adsorbates, as Eq. (2) in the main text suggests, implying the universal adsorption behavior on TMs and alloys. Moreover, the DFT-calculated prefactors $\mu_1$ and $\mu_2$ for adsorption at all considered adsorption sites (up to five) of TMs, NSAs, and BAs, and at the top site of HEAs are consistent with the predictions by Eq. (2) in the main text (Tables I, and S1-S3). It is noteworthy that for the OH adsorption at the bridge site of HEAs, the prefactor $\mu_1$ fulfills the prediction by Eq. (2) in the main text, while the prefactor $\mu_2$ [$\mu_2 = 3/5 \times (X+1)/(X_m+1)$] is three times of that at the top site [$\mu_2 = 1/5 \times (X+1)/(X_m+1)$] (see Tables S5 and S6). This indicates that the contribution of geometric effect to the OH adsorption energy at the bridge site of HEAs is greater than that at the top site.

In this study, we have studied the adsorption energy, activation energy, and reaction energy on TMs and alloys obtained by the different (semi-)local functionals including PBE, RPBE, PW91, BEEF-vdW and PBE-vdW functionals (see Figs. 1 and 2 in the main text and Figs. S5, S7-S26, S29, S30, S32, S33 and S35) [5–17]. It is encouraging that all the adsorption energies on TMs and alloys obey our scheme by Eqs. (2-4) in the main text and can be predicted by our scheme on equal footing (Fig. 3d in the main text), indicating that our scheme is independent on the choice of the (semi-)local functionals.

## Note S7: The activation energy, reaction energy and catalytic activity on TMs and alloys.

To identify the accuracy of our scheme in predicting the reactivity at surfaces, we revisit several widely-studied reactions on TMs and alloys, including the decomposition of $CH_4$, $NH_3$, $N_2$ and $H_2O$, thermochemical formation of $H_2O$ and $H_2$, decolorization reaction, $CO_2$ reduction reaction ($CO_2$RR), hydrogen evolution reaction (HER), oxygen reduction reaction (ORR), and oxygen evolution reaction (OER). We have studied the activation energy of 10 different reaction pathways including $CH_3 \rightarrow CH_2 + H$, $CH_2 \rightarrow CH + H$, $NH_3 \rightarrow NH_2 + H$, $NH_2 \rightarrow NH + H$, $NH \rightarrow N + H$, $N_2 \rightarrow 2N$, $H_2O \rightarrow OH + H$, $OH \rightarrow O + H$, $OH + H \rightarrow H_2O$, and $2H \rightarrow H_2$ on TMs, NSAs and HEAs (Figs. S29, S32, and S35) [9,10,15–17], the reaction energy of 8 different reaction pathways including $CH_4 \rightarrow CH_3 + H$, $CH_3 \rightarrow CH_2 + H$, $CH_2 \rightarrow CH + H$, $CH \rightarrow C + H$, $NH_3 \rightarrow NH_2 + H$, $NH_2 \rightarrow NH + H$, $NH \rightarrow N + H$, $OH \rightarrow O + H$ on TMs and BAs (Figs. S30 and S33) [15,17], and the experimental- and DFT-estimated catalytic activity (current density, onset potential, conversion efficiency, decoloration time, overpotential, Tafel slope and turnover frequency) towards decolorization reaction, $CO_2$RR, HER, ORR, OER, and $NH_3$ decomposition on TMs, NSAs, BAs, and HEAs (Figs. S31, S34, S38 and S39) [30–39]. Encouragingly, our scheme is effective in capturing all these activation energies, reaction energies, and reaction activity: the predicted MAE is about 0.12 eV for the activation energies and 0.17 eV for the reaction energies (Fig. S40), all of which are smaller than the approximate error of (semi-)local functionals, ±0.2 eV, while the predicted catalytic activity deviates less than 8%. Note that the electronic descriptor for the experimentally synthetic BAs and HEAs is obtained by using the geometric average of the stoichiometric ratio of the different components as the specific surface sites are uncertain. Nevertheless, this simple method is sufficiently accurate in describing the considered catalytic activity (see Figs. S34a-c, S38 and S39). These results demonstrate that our scheme is not only accurate for predicting the adsorption energy on TMs and alloys but also effective for directly characterizing the reactivity at surfaces, and thus can be used for the design of advanced alloy catalysts. According to the Brønsted–Evans–Polanyi (BEP) [40] relation, the activation energy is linearly related to the reaction energy of the reaction pathways, which corresponds to the difference between the adsorption energy of the reactants and products. As our model can determine the adsorption energy within the accuracy of DFT (semi-)local functionals, our model is effective in determining the activation energy and reaction energy. It is noteworthy that HEAs can break the BEP relation [40,41] because the reactants, transition states and products interact with the surface atoms with distinct electronic properties (Fig. S36). Nevertheless, our scheme can determine the adsorption energy and activation energy on HEAs well (Figs. S35 and S37), since it depends on the specific active center and adsorption site. These results strongly support the effectiveness and reliability of our model for the prediction of reactivity on TMs and alloys.

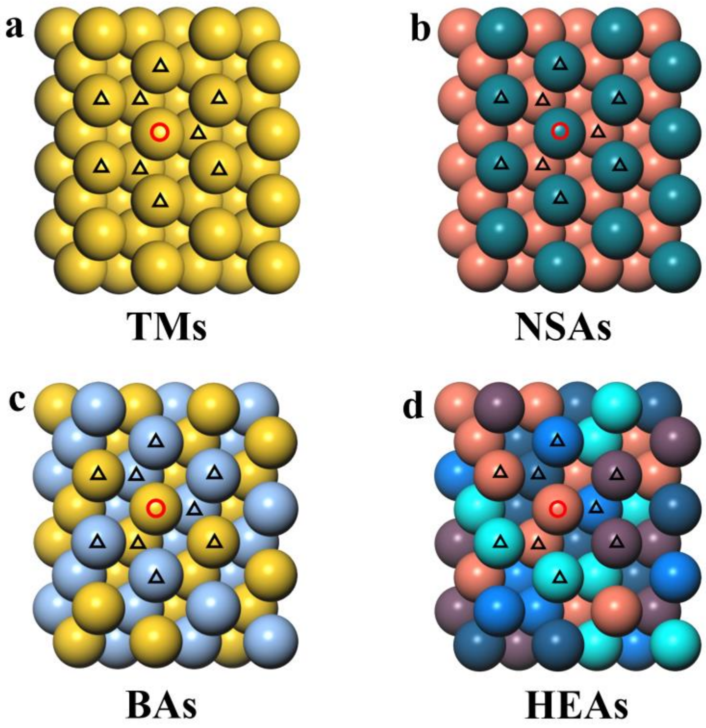


FIG. S1. The atomic structures of (111) surface of TMs (a), NSAs with the topmost layer being the alloying element (b), BAs with the stoichiometric ratio of 1 between the two components (c), and HEAs (d). The red circle and black triangle correspond to the adsorption site and its nearest neighbors. For NSAs and BAs, the adsorption-site effect of alloying denotes the change of the chemical composition of the adsorption site and the surrounding atoms that are the same as the adsorption site, while the environment effect of alloying does the change of the chemical properties of the surrounding atoms that are different from the adsorption site. For HEAs, the adsorption-site effect of alloying denotes the change of the chemical composition of the adsorption site with the fixed surrounding properties, whereas the environment effect of alloying does the change of the chemical properties of the nearest neighbors with the fixed adsorption-site properties.

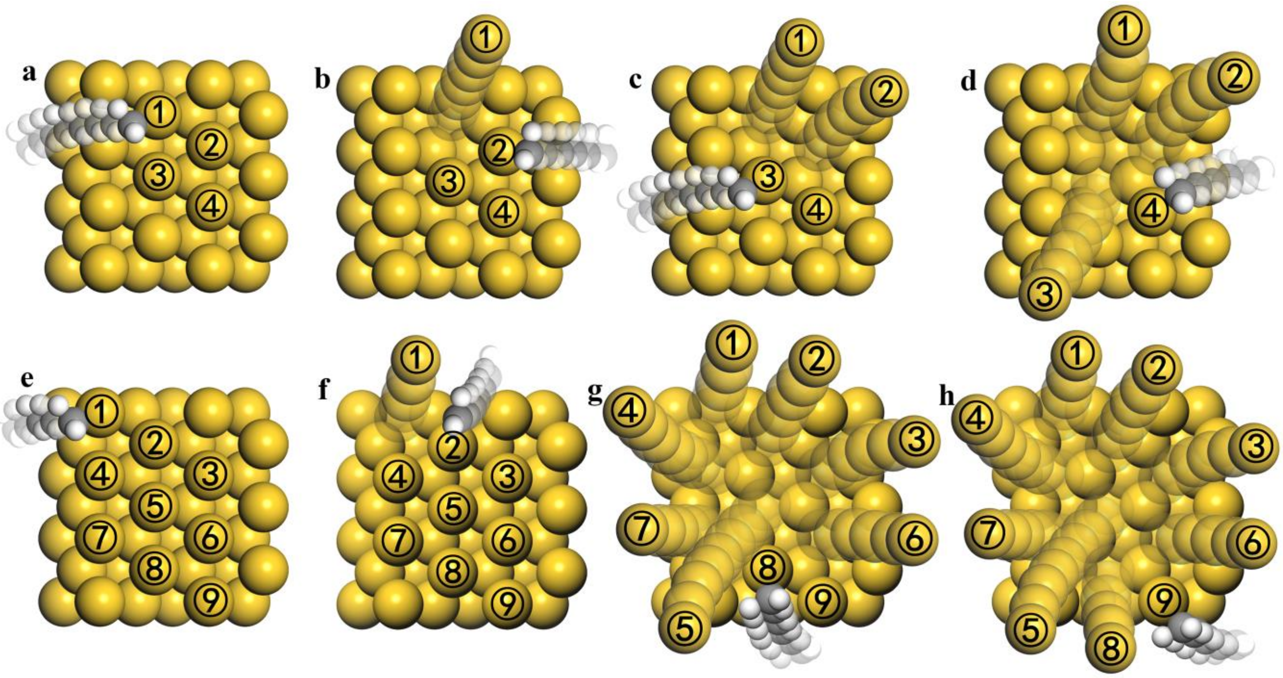


FIG. S2. The schematic illustration of surface adsorption in dissolution on TMs with (2 ×2) and (3 ×3) supercells. The symbols ①-⑨ correspond to the dissolution order of surface atoms and the corresponding adsorption order as the dissolution proceeds. (a)-(d), (2 ×2) supercell. (e)-(h), (3 ×3) supercell.

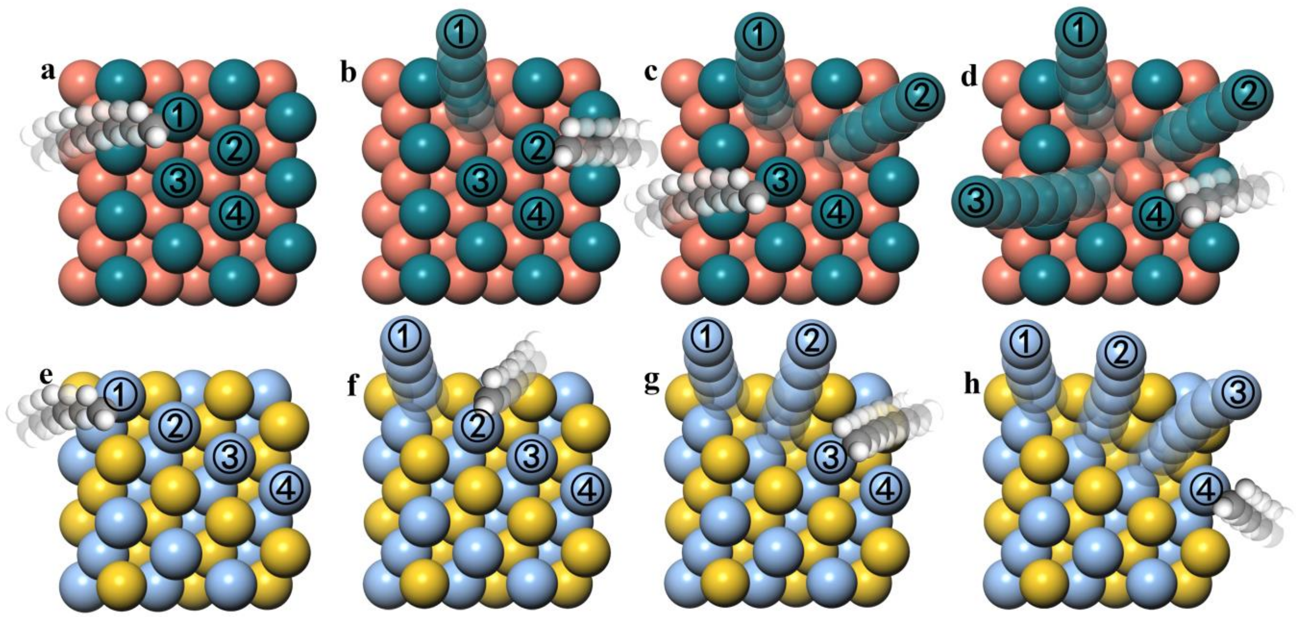


FIG. S3. The schematic illustration of surface adsorption in dissolution on NSAs and BAs. The symbols ①-④ correspond to the dissolution order of surface atoms and the corresponding adsorption order as the dissolution proceeds. (a)-(d), NSAs. (e)-(h), BAs.

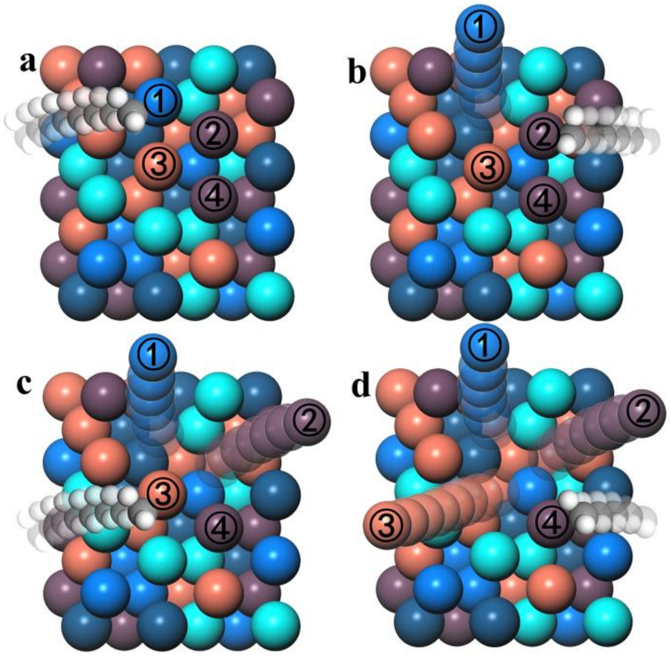


FIG. S4. The schematic illustration of surface adsorption in dissolution on HEAs. The symbols ①-④ correspond to the dissolution order of surface atoms and the corresponding adsorption order as the dissolution proceeds.

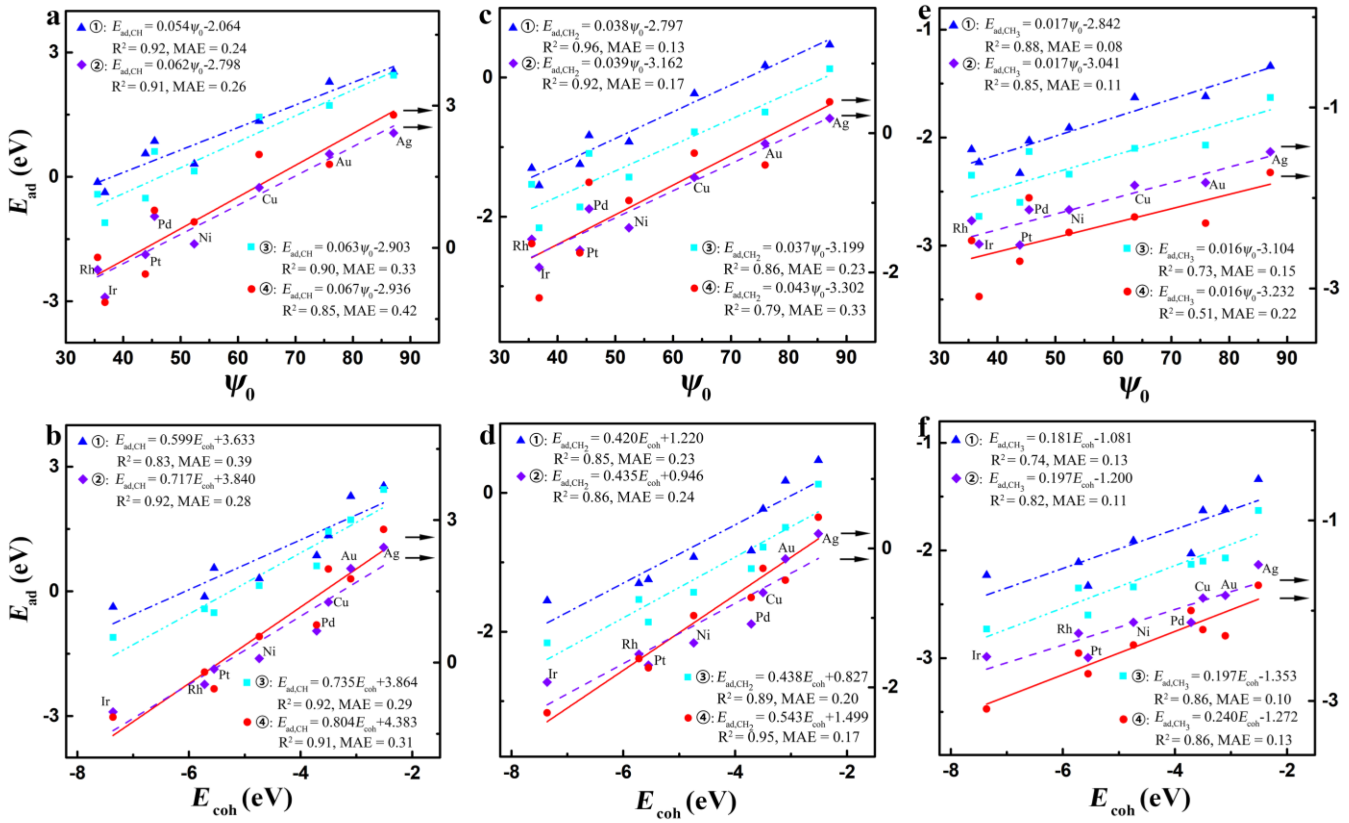


FIG. S5. Comparison between the electronic descriptor $\psi_0$ and cohesive energy $E_{coh}$ in describing the adsorption energy of C-based species on TM(111) surface in dissolution with (2 × 2) supercell. (a) and (b), CH. (c) and (d), $CH_2$. (e) and (f), $CH_3$ [6]. Note that the data for CH and $CH_2$ adsorption are calculated by PBE functional while those for $CH_3$ adsorption are calculated by RPBE functional.

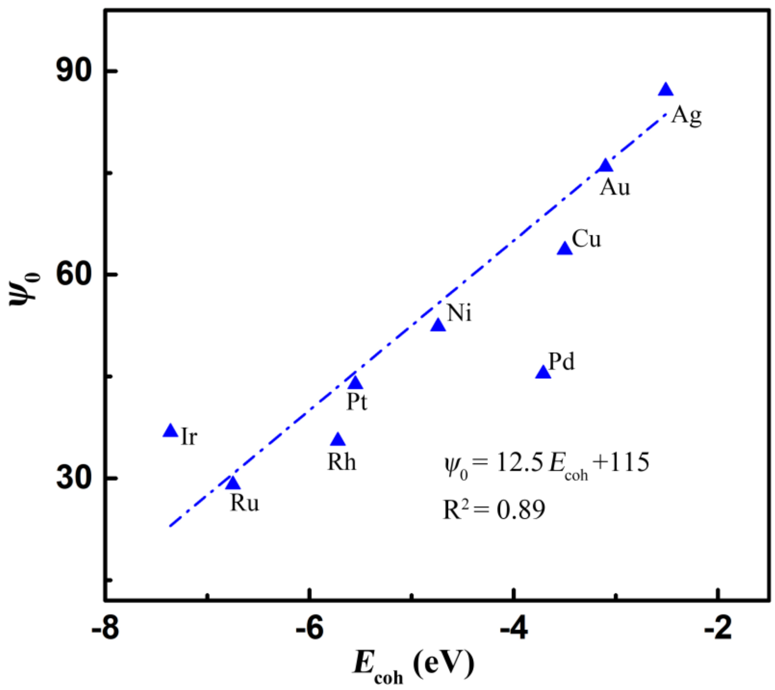


FIG. S6. The correlation between the cohesive energy ($E_{coh}$) of bulk atoms for TMs and the electronic descriptor $\psi_0$ [42]. Note that Pd is taken as an outlier in the linear fit.

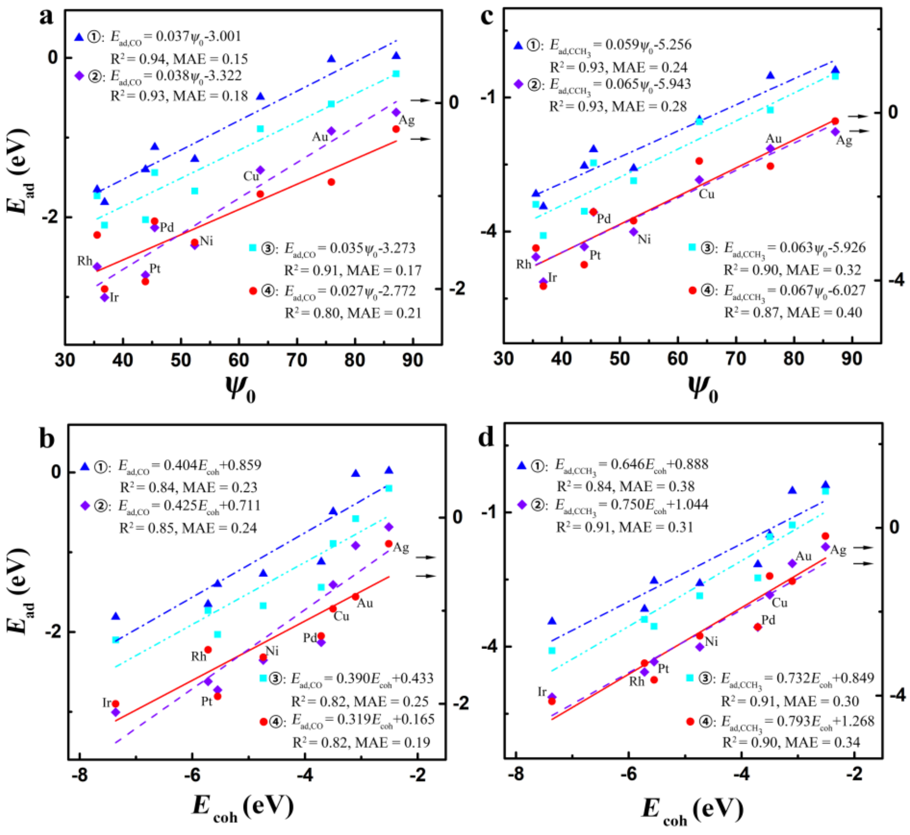


FIG. S7. Comparison between the electronic descriptor $\psi_0$ and cohesive energy $E_{coh}$ in describing the adsorption energy of C-based species on TM(111) surface in dissolution with (2 × 2) supercell. (a), CO [6]. (b), $CCH_3$. Note that the data for CO adsorption are calculated by RPBE functional while those for $CCH_3$ adsorption are calculated by PBE functional.

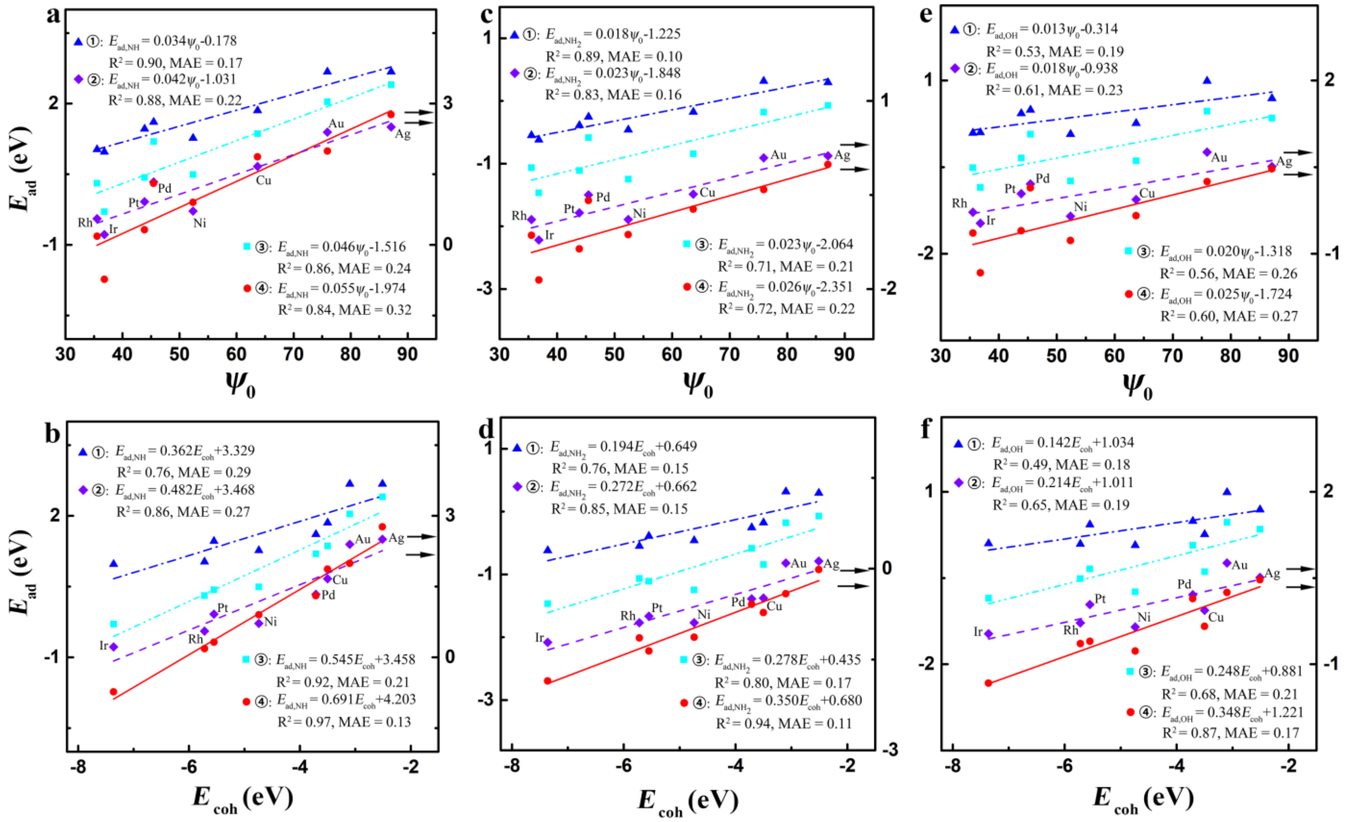


FIG. S8. Comparison between the electronic descriptor $\psi_0$ and cohesive energy $E_{coh}$ in describing the adsorption energy of N- and O-based species on TM(111) surface in dissolution with (2 × 2) supercell. (a) and (b), NH. (c) and (d), $NH_2$. (e) and (f), OH [6]. Note that the data for NH and $NH_2$ adsorption are calculated by PBE functional while those for OH adsorption are calculated by RPBE functional.

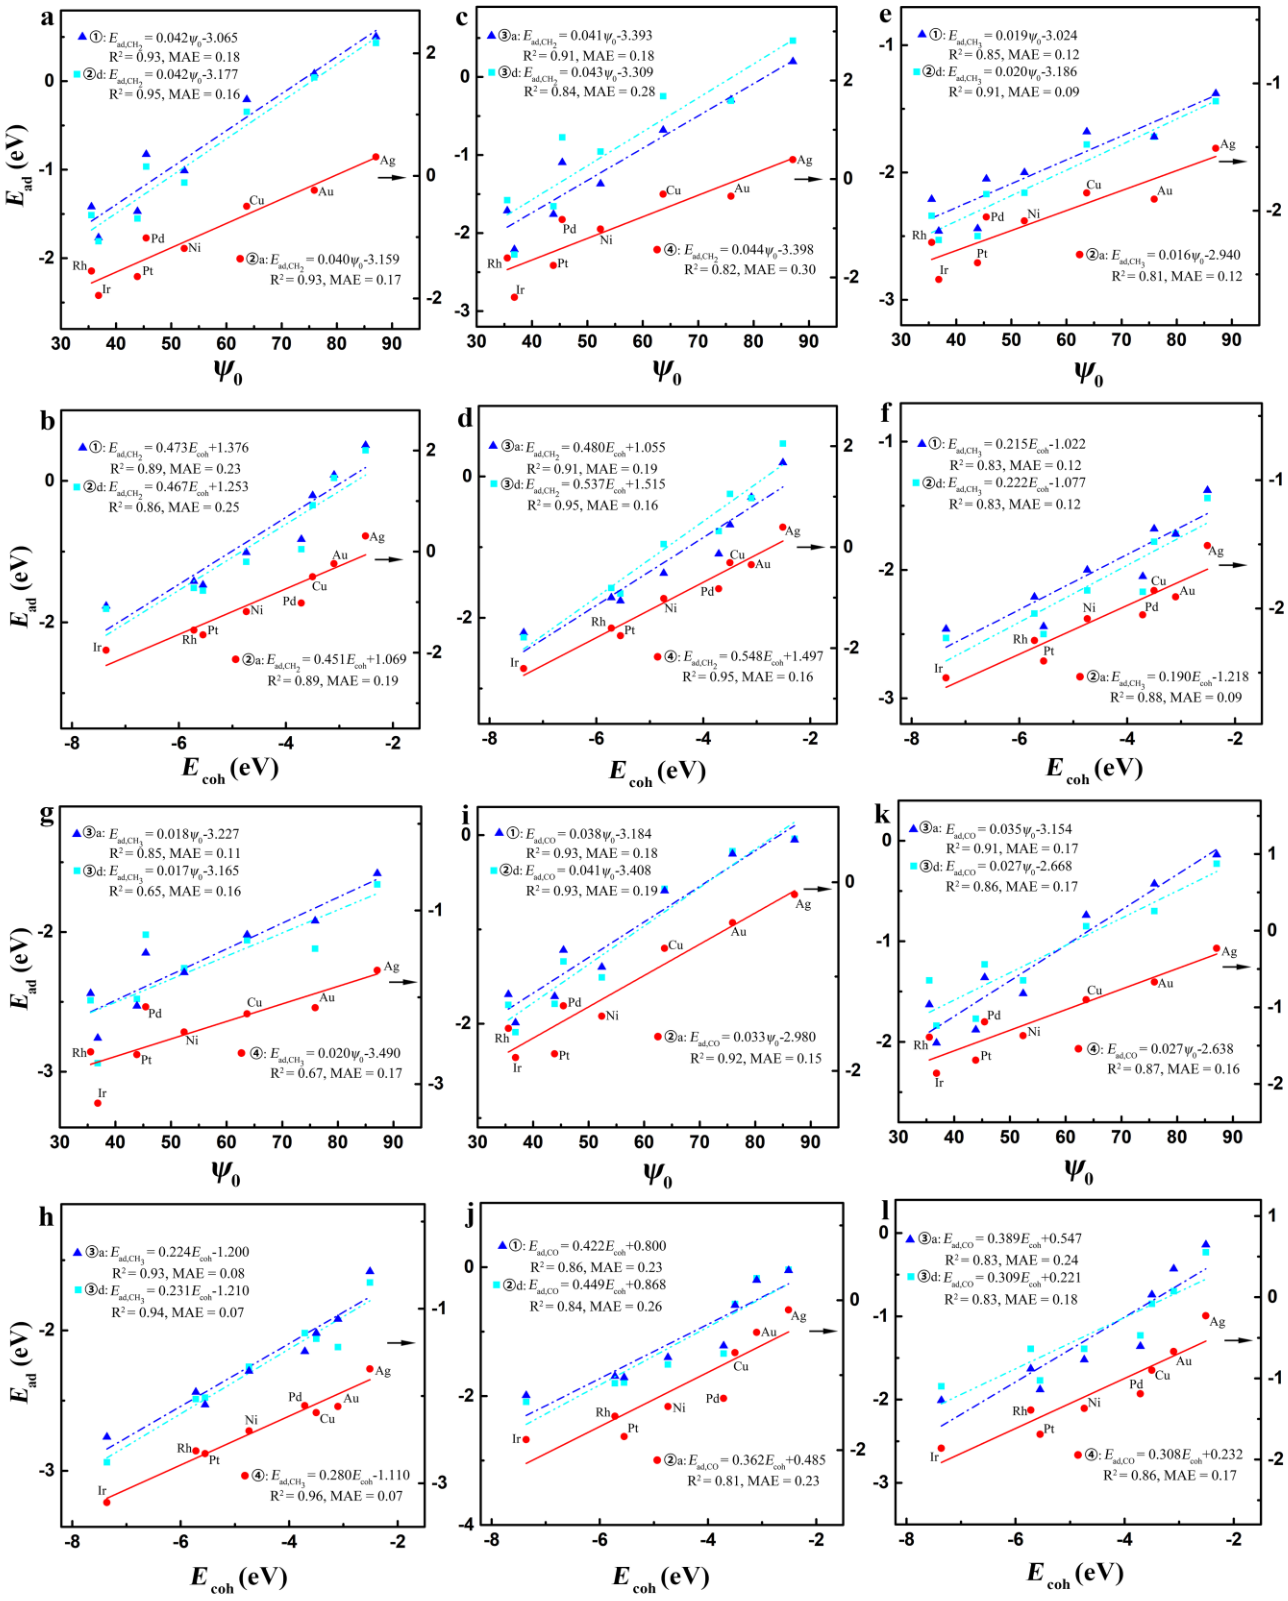


FIG. S9. Comparison between the electronic descriptor $\psi_0$ and cohesive energy $E_{coh}$ in describing the adsorption energy of C-based species on TM(100) surface in dissolution with (2 ×2) supercell. (a)-(d), $CH_2$. (e)-(h), $CH_3$ [6]. (i)-(l), CO [6]. Note that the data for $CH_2$ adsorption are calculated by PBE functional while those for $CH_3$ and CO adsorption are calculated by RPBE functional.

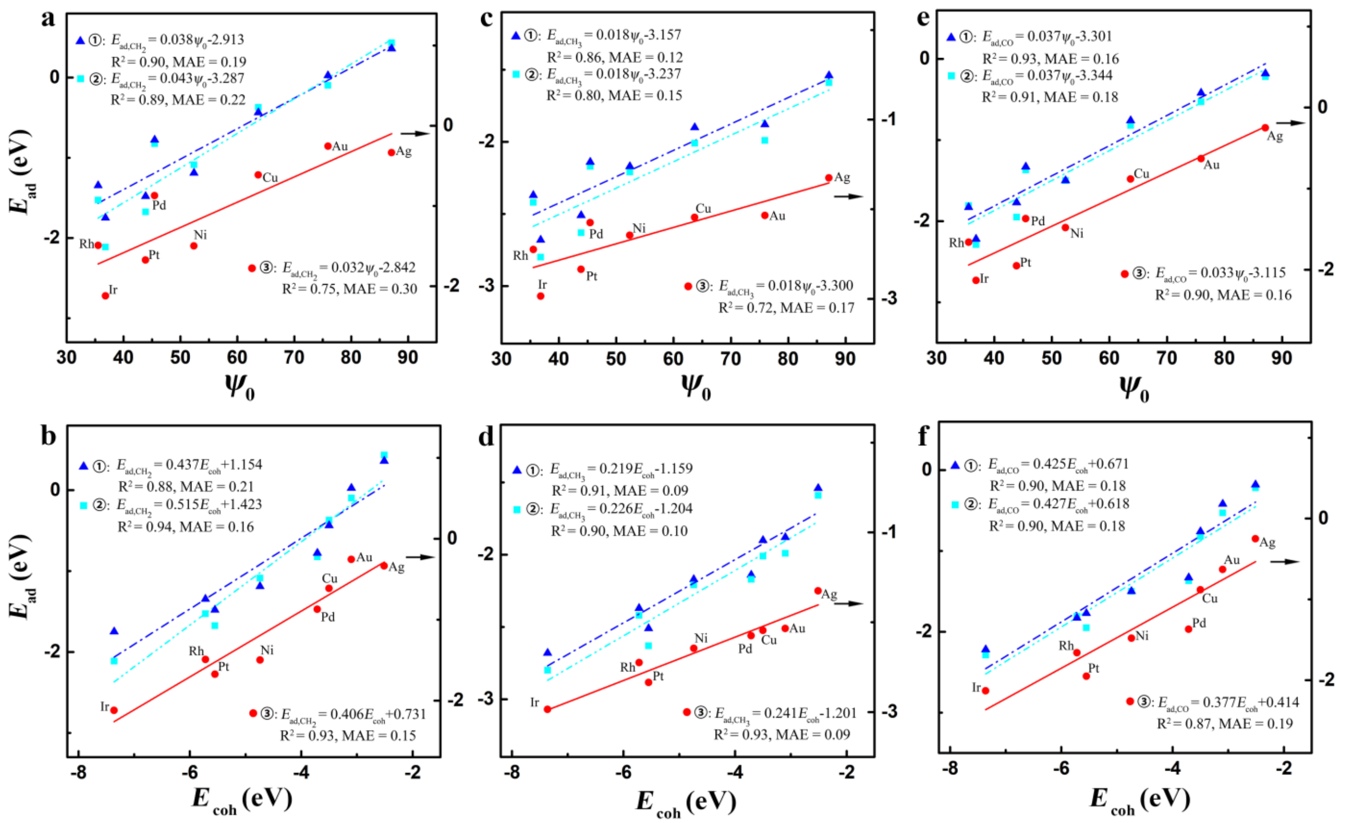


FIG. S10. Comparison between the electronic descriptor $\psi_0$ and cohesive energy $E_{coh}$ in describing the adsorption energy of C-based species on TM(211) surface in dissolution with (1 × 3) supercell. (a) and (b), $CH_2$. (c) and (d), $CH_3$ [6]. (e) and (f), CO [6]. Note that the data for $CH_2$ adsorption are calculated by PBE functional while those for $CH_3$ and CO adsorption are calculated by RPBE functional.

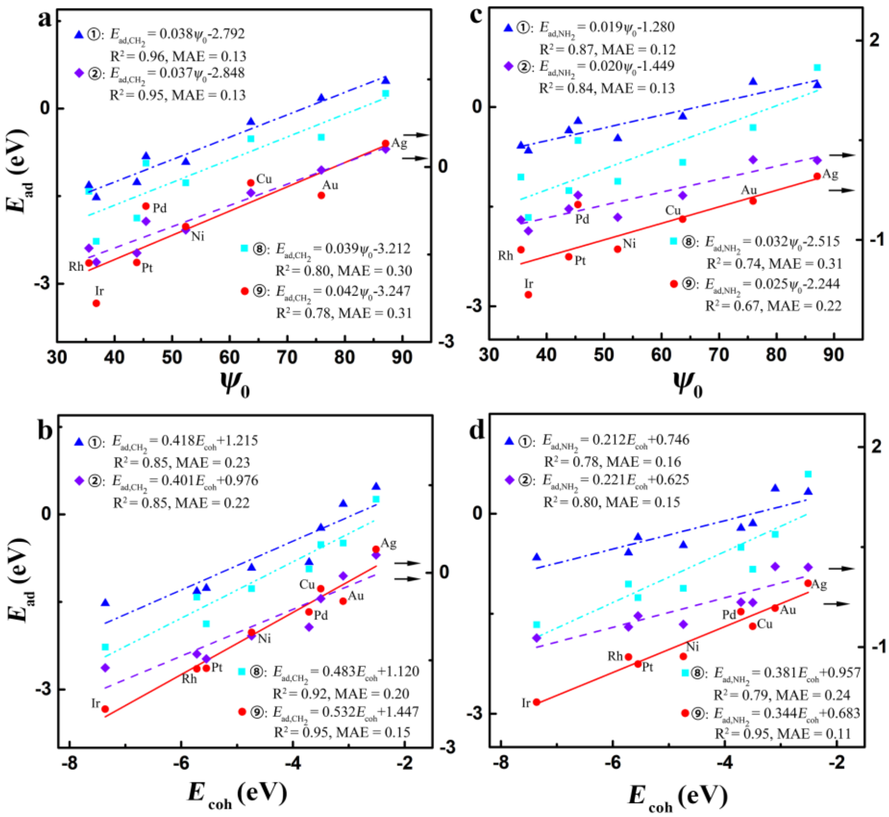


FIG. S11. Comparison between the electronic descriptor $\psi_0$ and cohesive energy $E_{coh}$ in describing the adsorption energy on TM(111) surface in dissolution with (3 × 3) supercell. (a) and (b), $CH_2$. (c) and (d), $NH_2$. All data are calculated with PBE functional.

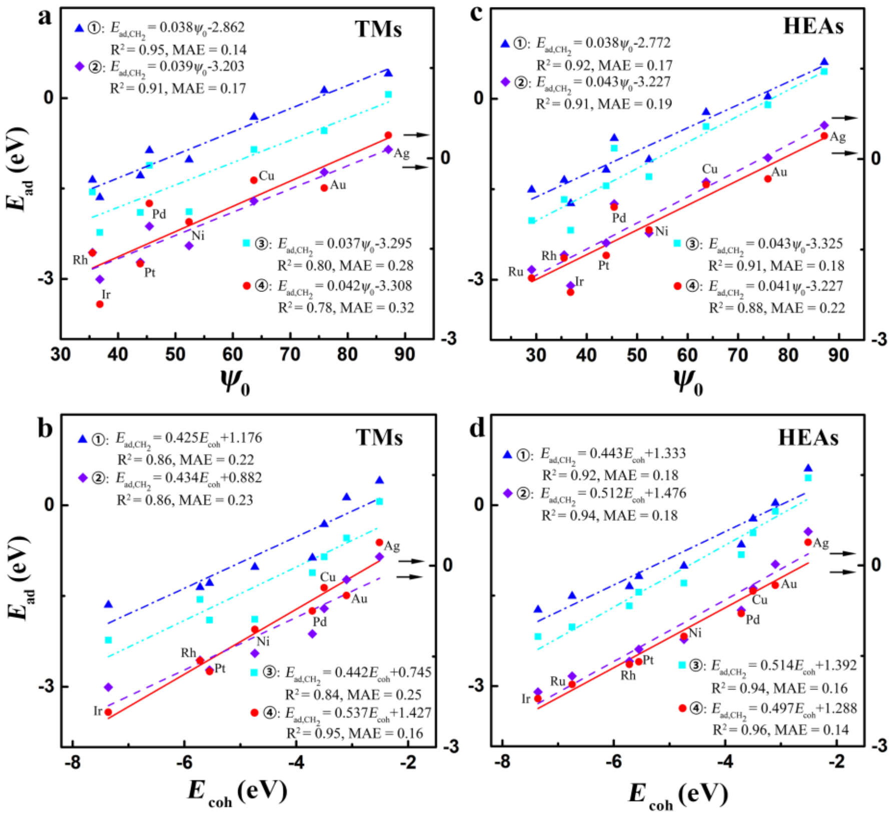


FIG. S12. Comparison between the electronic descriptor $\psi_0$ and cohesive energy $E_{coh}$ in describing the adsorption energy of $CH_2$ on (111) surface of TMs with (2 × 2) supercell and RuRhIrPdPt-based HEAs with (4 × 4) supercell in dissolution (a) and (b), TMs. (c) and (d), HEAs. All data are calculated with PW91 functional.

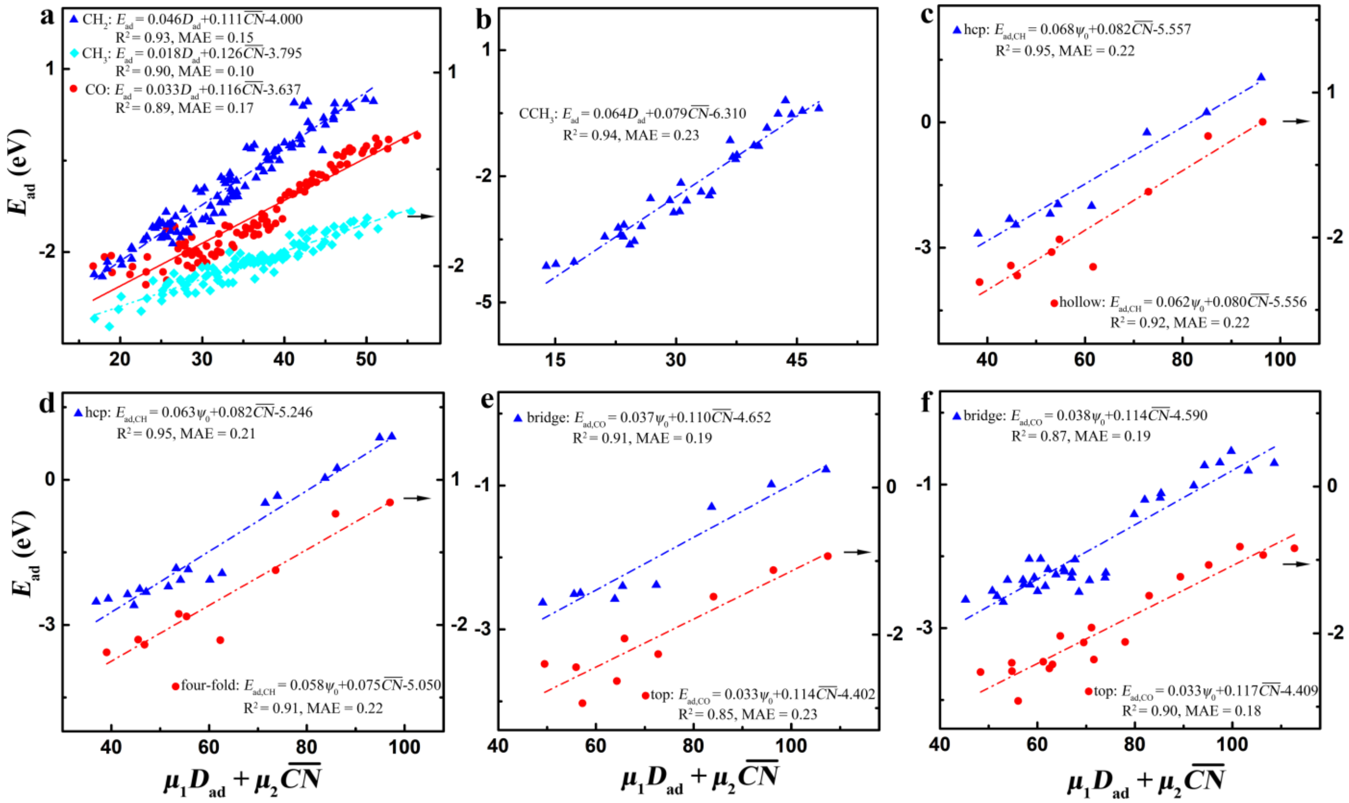


FIG. S13. Adsorption energies of the different adsorbates against the electronic and geometric descriptors on TMs. (a), $CH_2$, $CH_3$ [6] and CO [6] adsorption at the top site of (111), (100) and (211) surfaces in dissolution. Note that the data for $CH_2$ adsorption are calculated by PBE functional while those for $CH_3$ and CO adsorption are calculated by RPBE functional. (b), $CCH_3$ adsorption at the top site of (111) surface in dissolution with the data calculated by PBE functional. (c), CH adsorption at the hcp site of the undissolved (111) surface and the hollow site of the undissolved (100) surface with the data calculated by BEEF-vdW functional [7]. (d), CH adsorption at the hcp and four-fold sites of the undissolved (211) surface with the data calculated by BEEF-vdW functional [7]. (e), CO adsorption at the bridge site of the undissolved (100) surface and the top site of the undissolved (110) surface with the data calculated by BEEF-vdW functional [7]. (f), CO adsorption at the bridge and top sites of the undissolved (211) surface with the data calculated by BEEF-vdW functional [7]. Note that the data in subfigures (a) and (b) are calculated with (2 × 2) supercell for (111) and (100) surfaces and (1 × 3) supercell for (211) surface, while those in subfigures (c)-(f) are calculated with (3 × 3) supercell for (111) and (100) surfaces, (2 × 3) supercell for (110) surface, and (1 × 3) supercell for (211) surface.

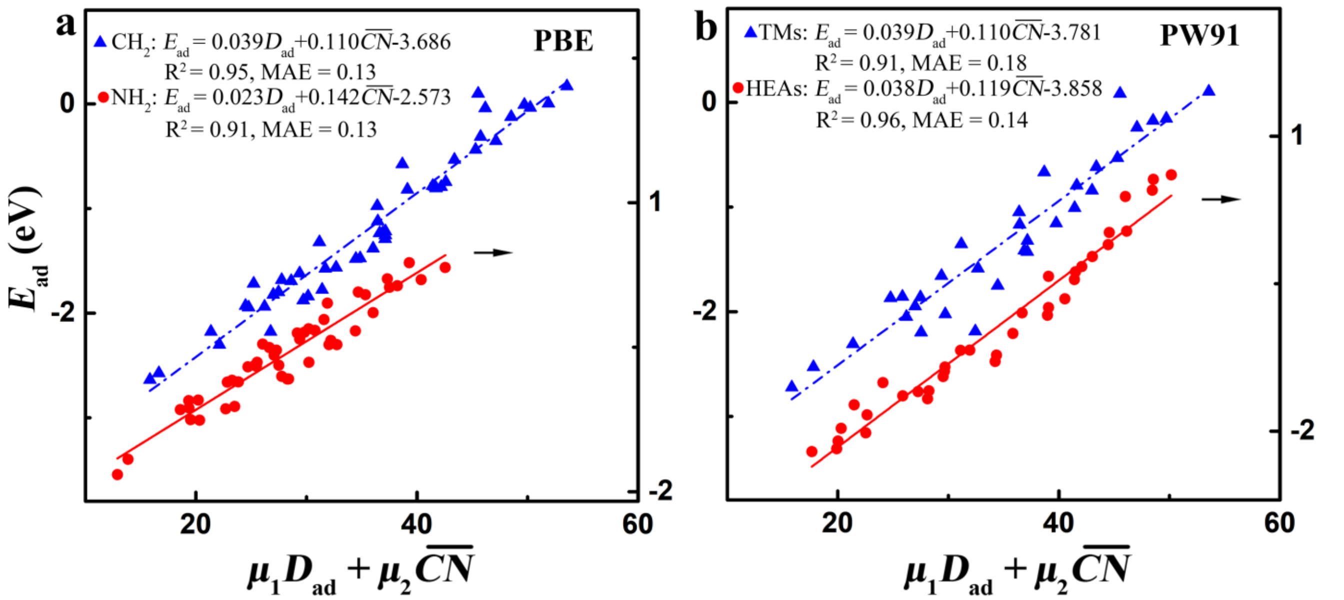


FIG. S14. Adsorption energies of the different adsorbates against the electronic and geometric descriptors on TMs and HEAs. (a), $CH_2$ and $NH_2$ adsorption at the top site of TM(111) surface with (3 × 3) supercell in dissolution with the data calculated by PBE functional. (b), $CH_2$ adsorption at the top site of TM(111) surface with (2 × 2) supercell and HEA(111) surface with (4 × 4) supercell in dissolution in the adsorption-site effect of alloying with the data calculated by PW91 functional.

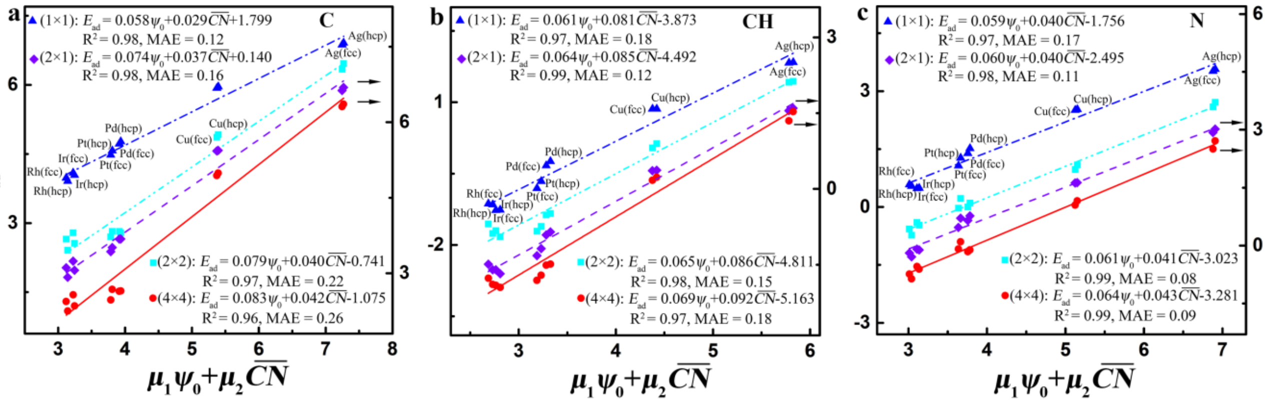


FIG. S15. Adsorption energies of the different adsorbates against the electronic and geometric descriptors on TM(111) surface with (1 × 1), (2 × 1), (2 × 2), and (4 × 4) supercells [8]. (a), C. (b), CH. (c), N. All data are calculated with BEEF-vdW functional.

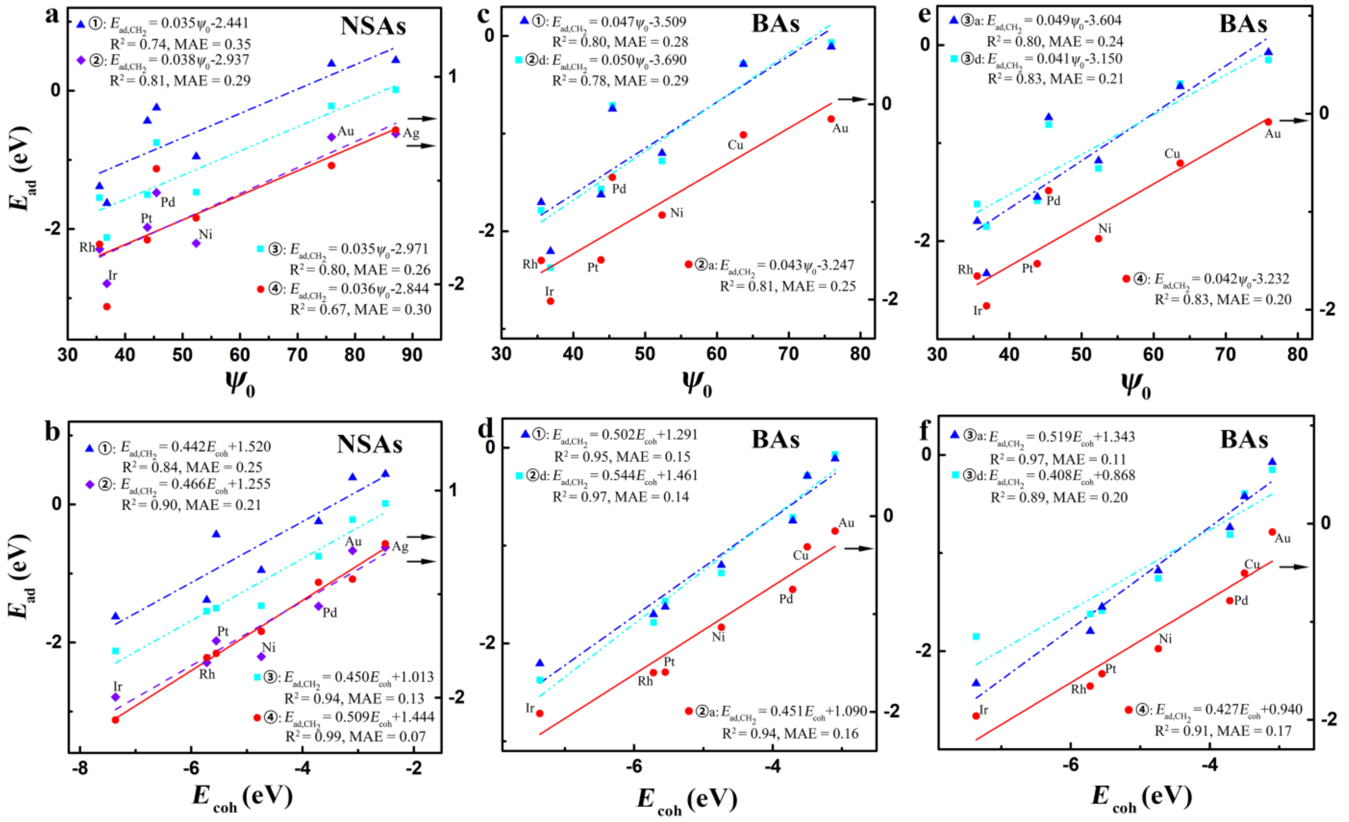


FIG. S16. Comparison between the electronic descriptor $\psi_0$ and cohesive energy $E_{coh}$ in describing the adsorption energy of $CH_2$ on (111) surface of Cu-based NSAs (a) and (b), and (100) surface of Ag-based BAs (c)-(f) in dissolution with (2 × 2) supercell. All data are calculated by PBE functional.

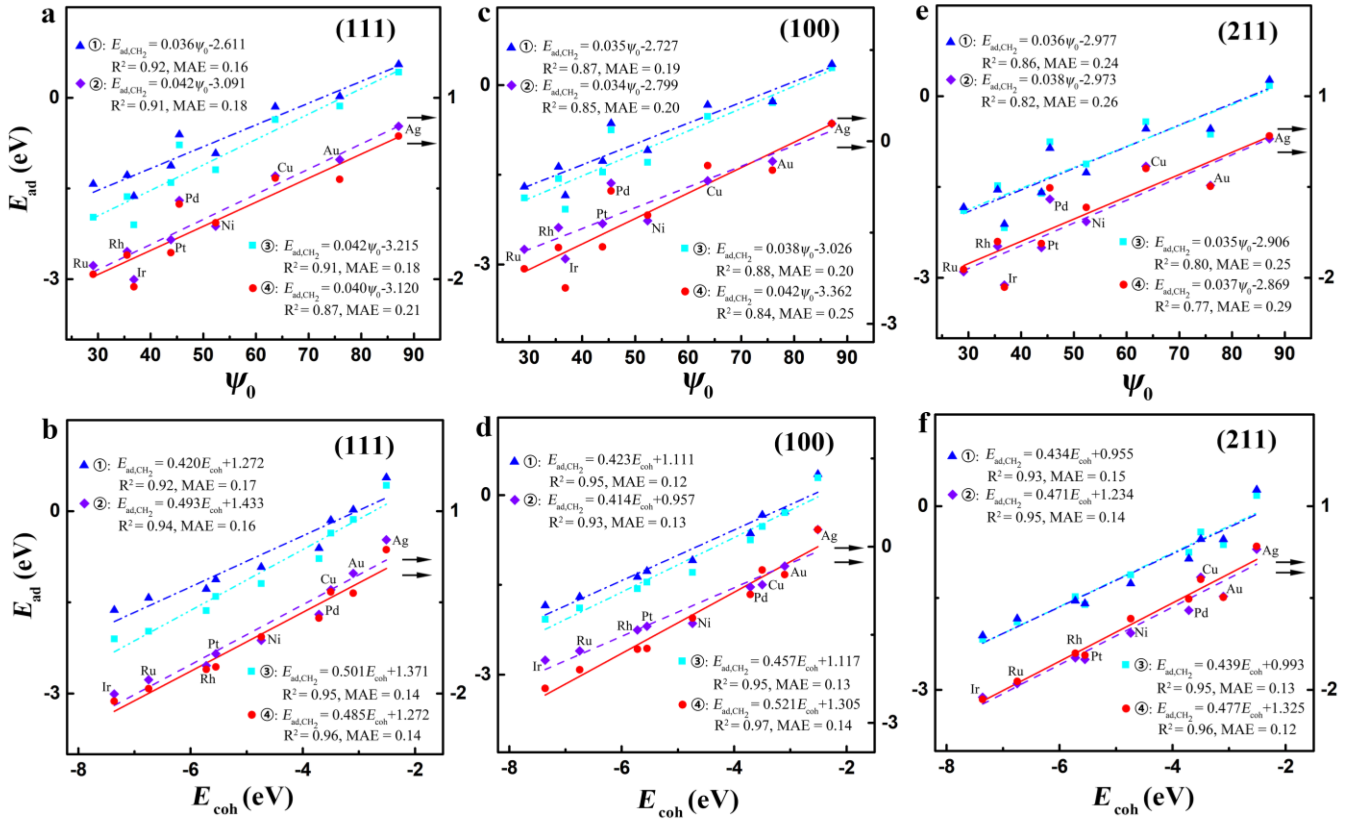


FIG. S17. Comparison between the electronic descriptor $\psi_0$ and cohesive energy $E_{coh}$ in describing the adsorption energy of $CH_2$ on RuRhIrPdPt-based HEAs in dissolution. (a) and (b), (111) surface with (4 × 4) supercell. (c) and (d), (100) surface with (4 × 4) supercell. (e) and (f), (211) surface with (2 × 4) supercell. All data are calculated by PBE functional.

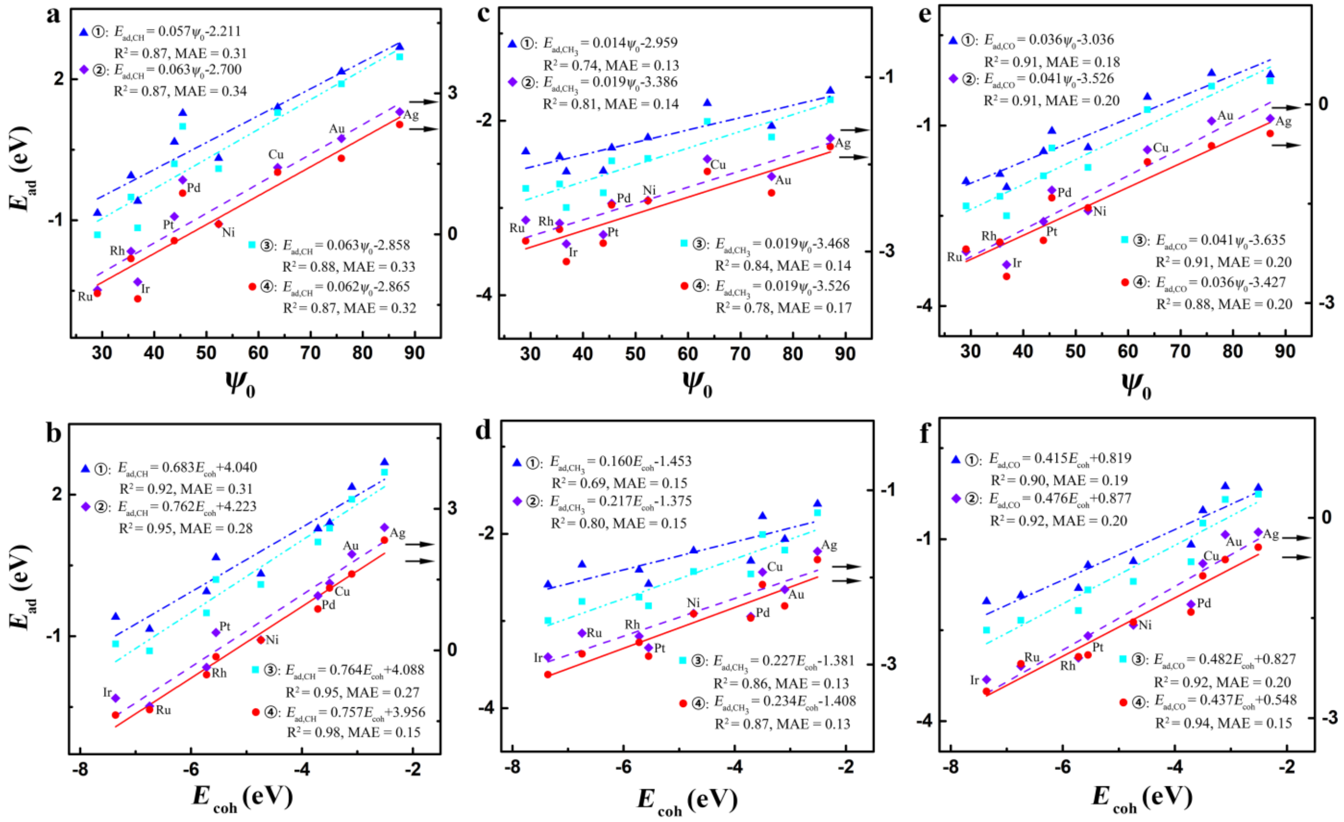

FIG. S18. Comparison between the electronic descriptor $\psi_0$ and cohesive energy $E_{coh}$ in describing the adsorption energy of C-based species on (111) surface of RuRhIrPdPt-based HEAs in dissolution with (4 × 4) supercell. (a) and (b), CH. (c) and (d), $CH_3$. (e) and (f), CO. All data are calculated by PBE functional.

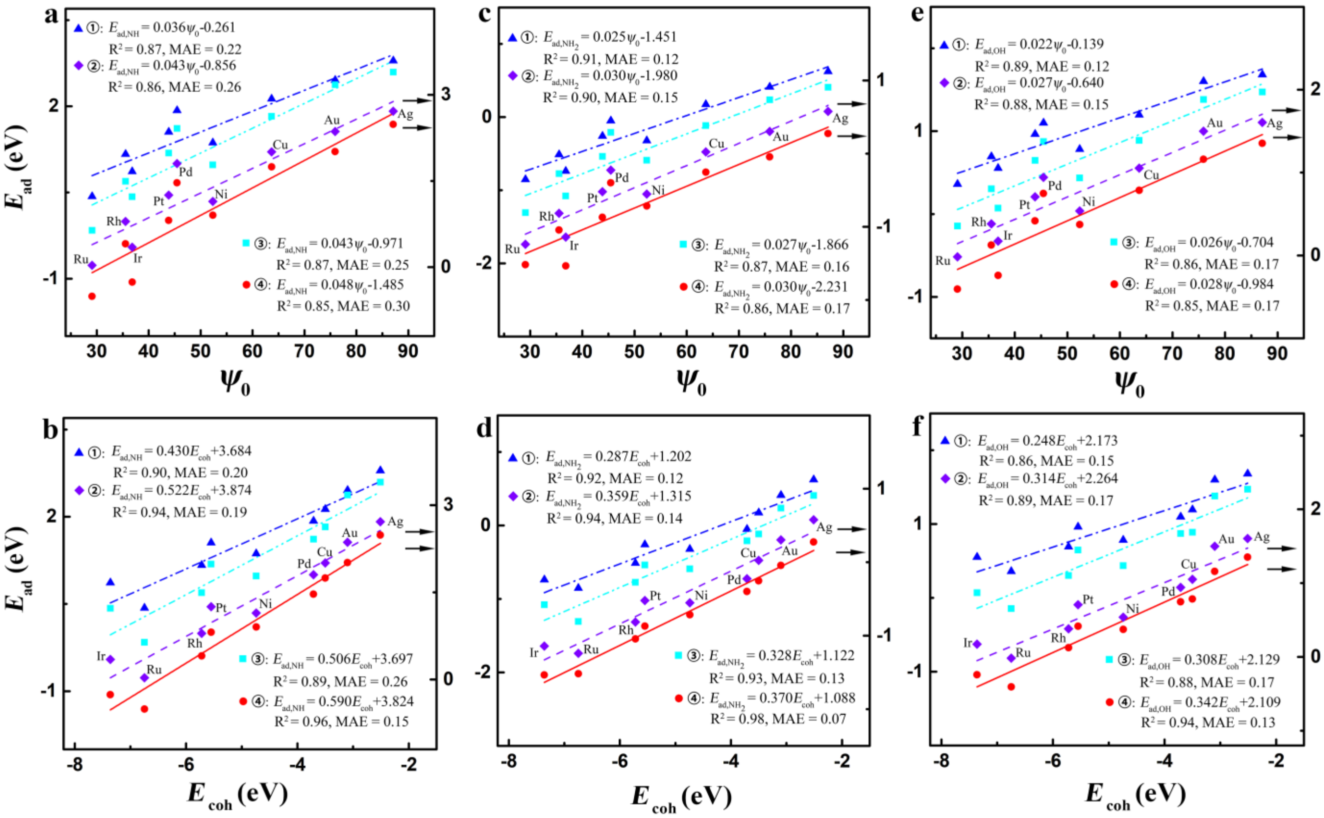


FIG. S19. Comparison between the electronic descriptor $\psi_0$ and cohesive energy $E_{coh}$ in describing the adsorption energy of N- and O-based species on (111) surface of RuRhIrPdPt-based HEAs in dissolution with (4 × 4) supercell. (a) and (b), NH. (c) and (d), $NH_2$. (e) and (f), OH. All data are calculated by PBE functional.

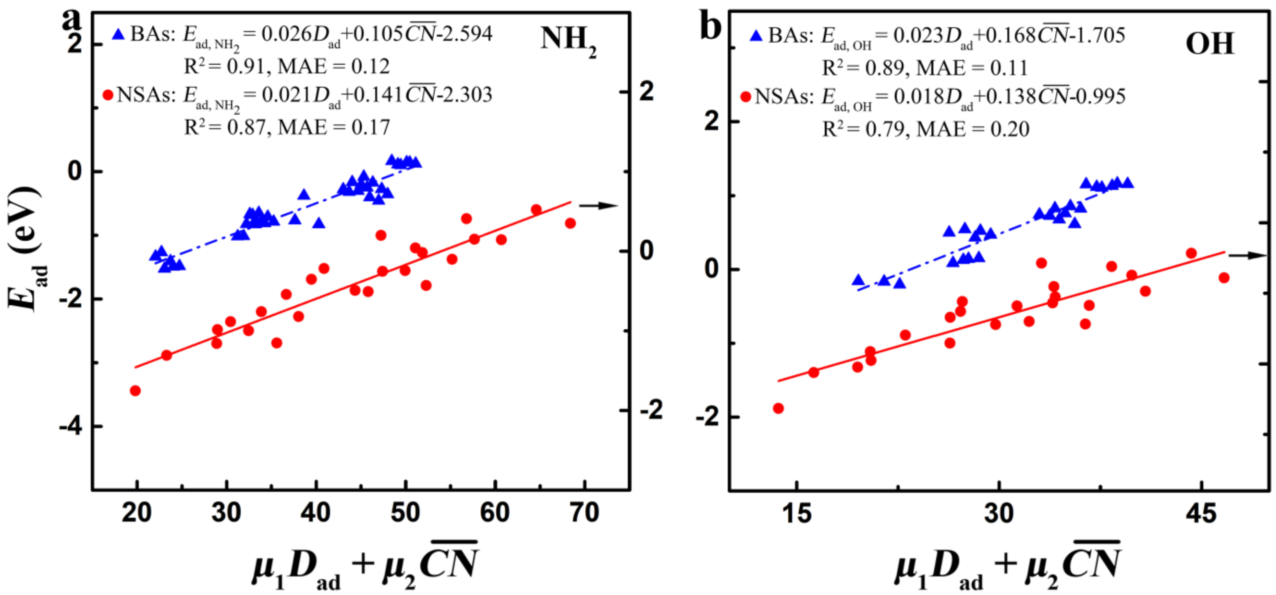


FIG. S20. Adsorption energies of $NH_2$ and OH against the electronic and geometric descriptors at the top site of (100) surface of Ag-based BAs and (111) surface of Cu-based NSAs in dissolution with (2 × 2) supercell in the adsorption-site effect of alloying. (a), $NH_2$. (b), OH. All data are calculated by PBE functional.

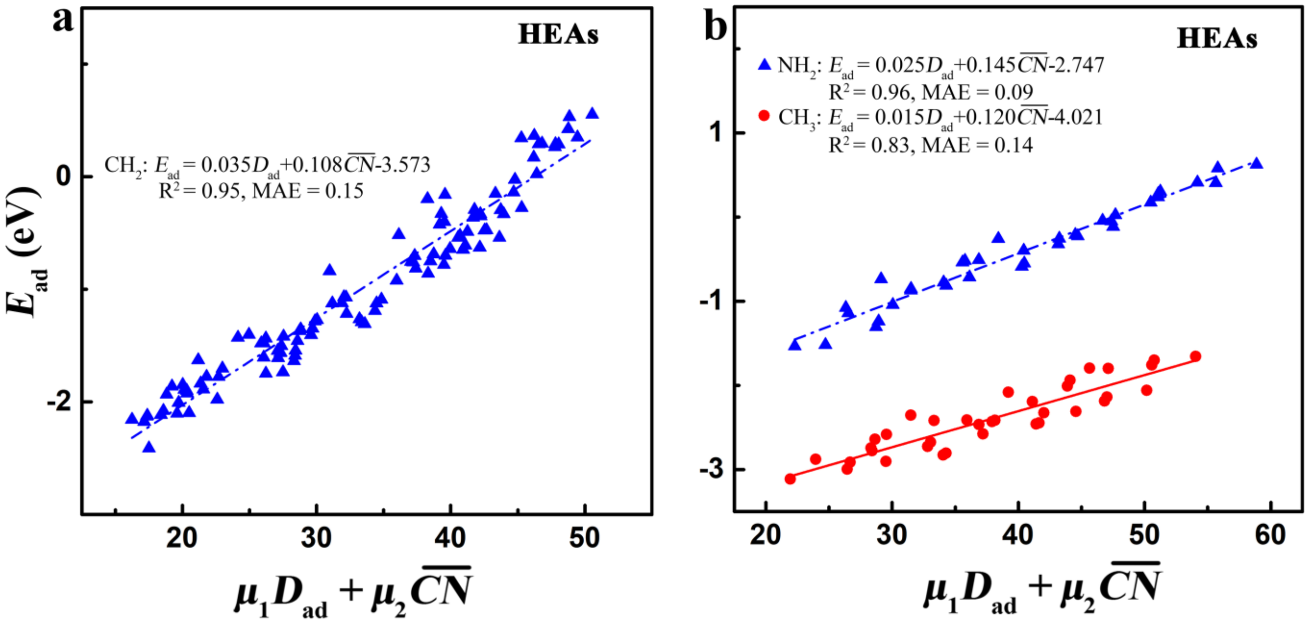


FIG. S21. Adsorption energies of the different adsorbates in dissolution against the electronic and geometric descriptors at the top site of RuRhIrPdPt-based HEAs in the adsorption-site effect of alloying. (a), $CH_2$ adsorption on (111), (100) and (211) surfaces of HEAs. (b), $NH_2$ and $CH_3$ adsorption on (111) surface of HEAs. All data are calculated by PBE functional. Note that (111) and (100) surfaces are modeled by (4 $\times$ 4) supercell while (211) surface is modeled by (2 $\times$ 4) supercell.

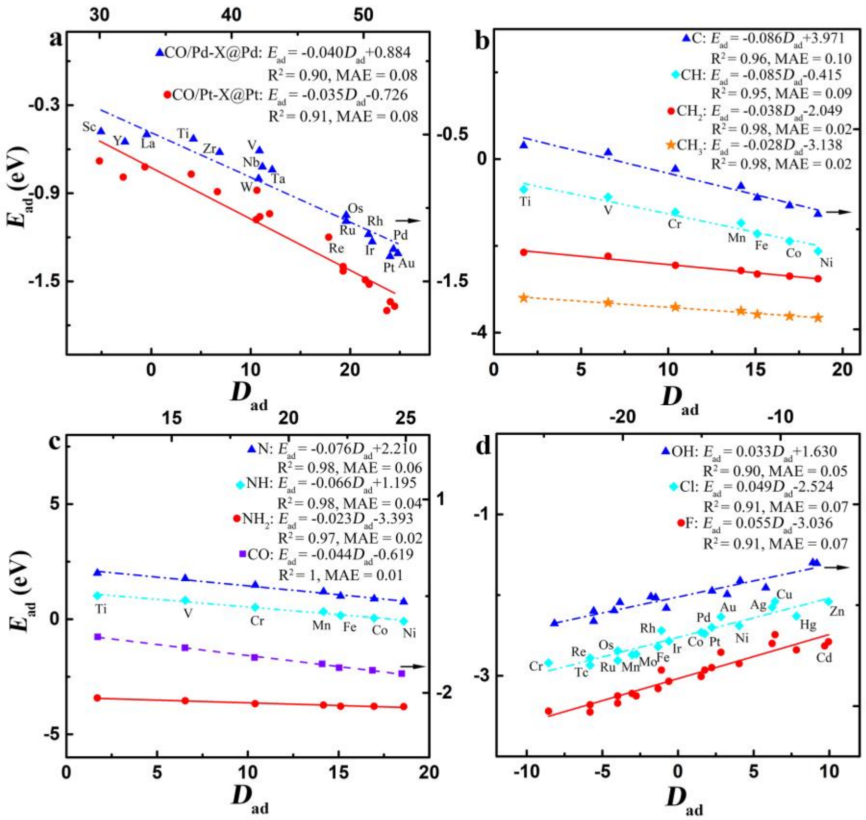


FIG. S22. Adsorption energies of the different adsorbates against the electronic descriptor at the top site of Pt- and Pd-based NSAs in the environment-effect of alloying. (a), CO adsorption on (100) surface with (4 × 2) supercell of Pt- and Pd-based NSAs [14]. (b)-(d), $CH_x$ ($x$ = 0-3), CO, $NH_x$ ($x$= 0-2) [11], OH [13], F and Cl [12] on (111) surface with (2 × 2) supercell of Pt-based NSAs. Note that the data for CO, and F and Cl in subfigures (a) and (d) are calculated by PBE functional while those for $CH_x$ ($x$ = 0-3), CO, $NH_x$ ($x$= 0-2), and OH in subfigures (b)-(d) are calculated by PW91 functional.

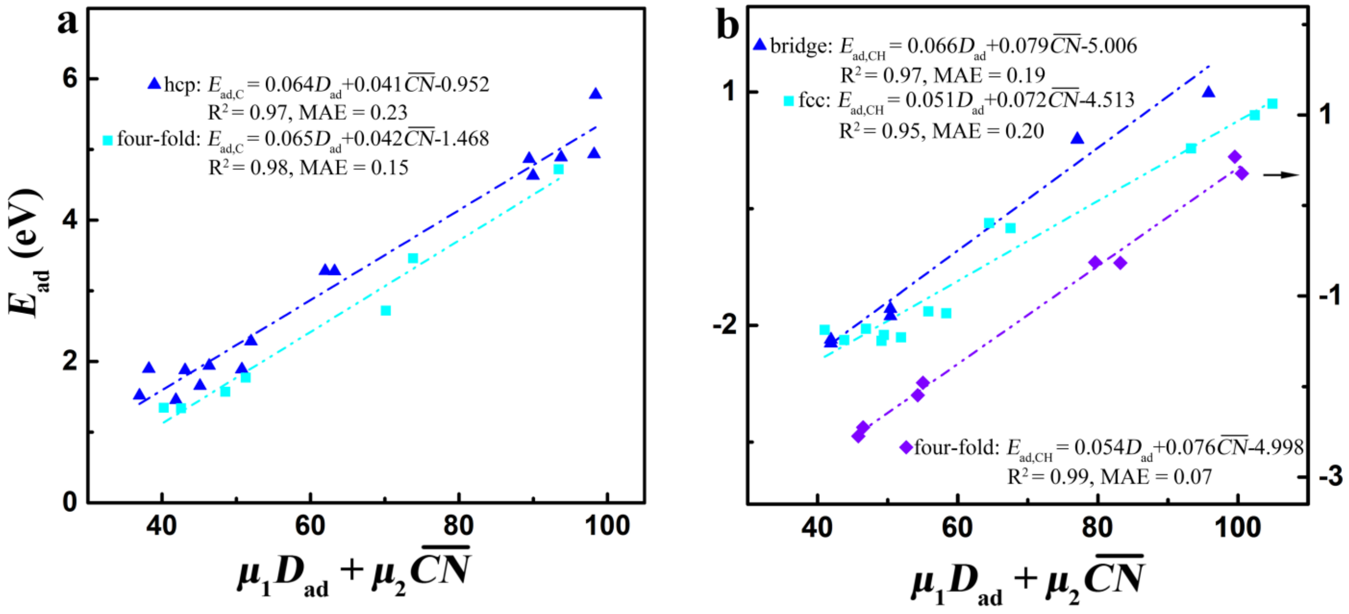


FIG. S23. Adsorption energies of C and CH against the electronic and geometric descriptors on AgAu, AgPd, IrRu, and PtRh BAs with the variable adsorption sites and surrounding environments in both the adsorption-site and environment effects of alloying [7]. (a), C adsorption at the hcp and four-fold sites of the undissolved (211) surface of BAs. (b), CH adsorption at the bridge, fcc and four-fold sites of the undissolved (211) surface of BAs. All data are calculated by BEEF-vdW functional and (211) surface is modeled by (1 × 2) supercell.

.

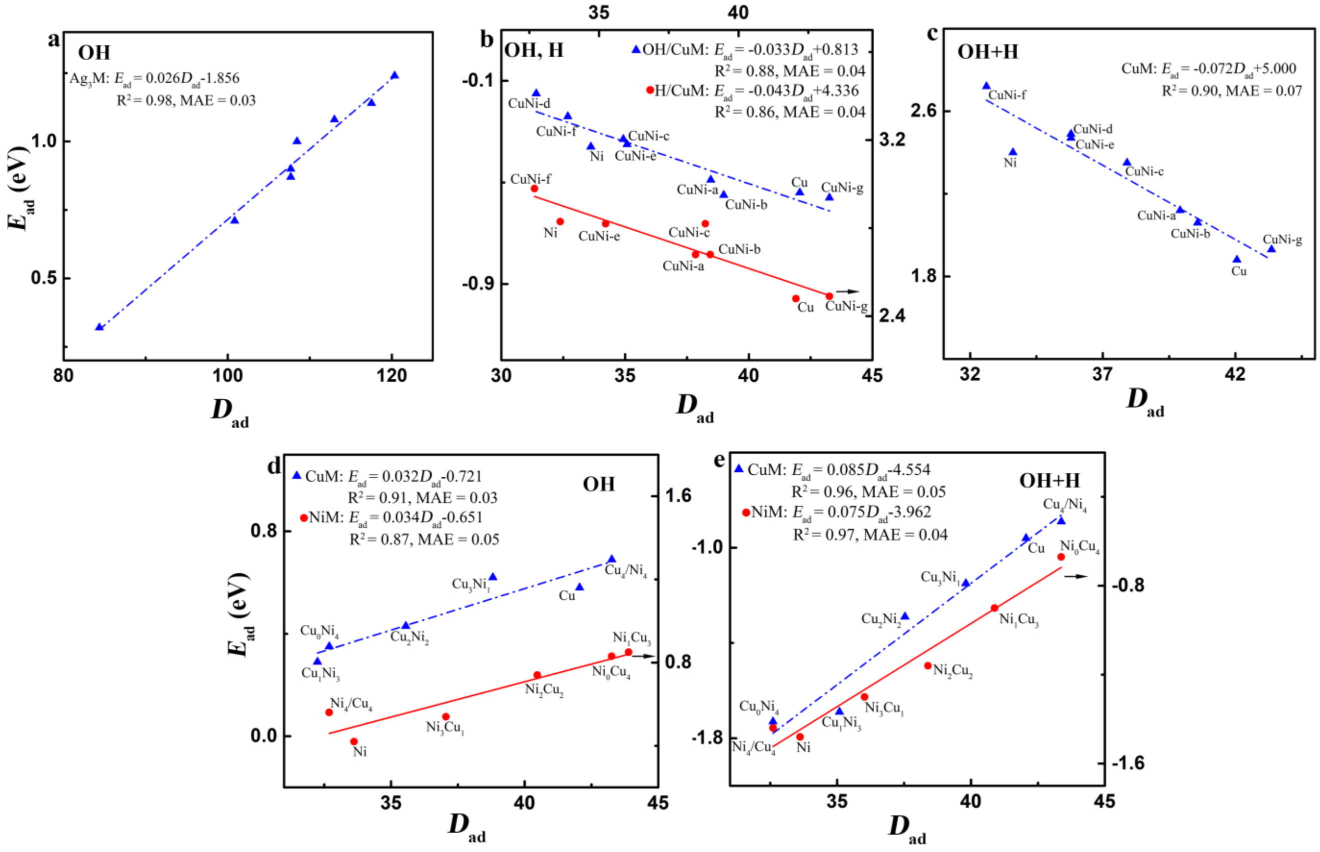


FIG. S24. Adsorption energies against the electronic descriptor on BAs and NSAs with the variable adsorption sites and surrounding environments in both the adsorption-site and environment effects of alloying. (a), OH adsorption at the different hcp sites of (111) surface with (2 × 2) supercell of Ag-based $Ag_3M$ (M = Cu, Pt, Pd, Rh and Ru) BAs with the data calculated by BEEF-vdW functional. Note that the data are accessible in Ref. [15] at https://www.catalysis-hub.org/energies. (b) and (c), OH and H adsorption and OH + H coadsorption at the fcc site of (111) surface with (3 × 3) supercell of Cu, Ni and Cu-based CuNi NSAs with the different Cu/Ni ratios [including one Ni atom in the topmost layer (CuNi-a), two Ni atoms in the topmost layer (CuNi-c), three Ni atoms in the topmost layer with the different distributions (CuNi-b, CuNi-d and CuNi-e), nine Ni atoms in the topmost layer (CuNi-f), and nine Ni atoms in the subsurface layer (CuNi-g)] with the data calculated by PW91 functional [10]. (d) and (e), OH adsorption at the fcc site and OH + H coadsorption at the fcc+hcp site of (111) surface with (2 × 2) supercell of Cu, Ni, Cu-based CuNi and Ni-based NiCu NSAs with the different Cu/Ni ratios [including Cu and Ni atoms in the topmost layer ($Cu_xNi_y$ and $Ni_xCu_y$) and Ni ($Cu_4/Ni_4$) or Cu ($Ni_4/Cu_4$) atoms in the subsurface layer] with the data calculated by PBE functional [9].

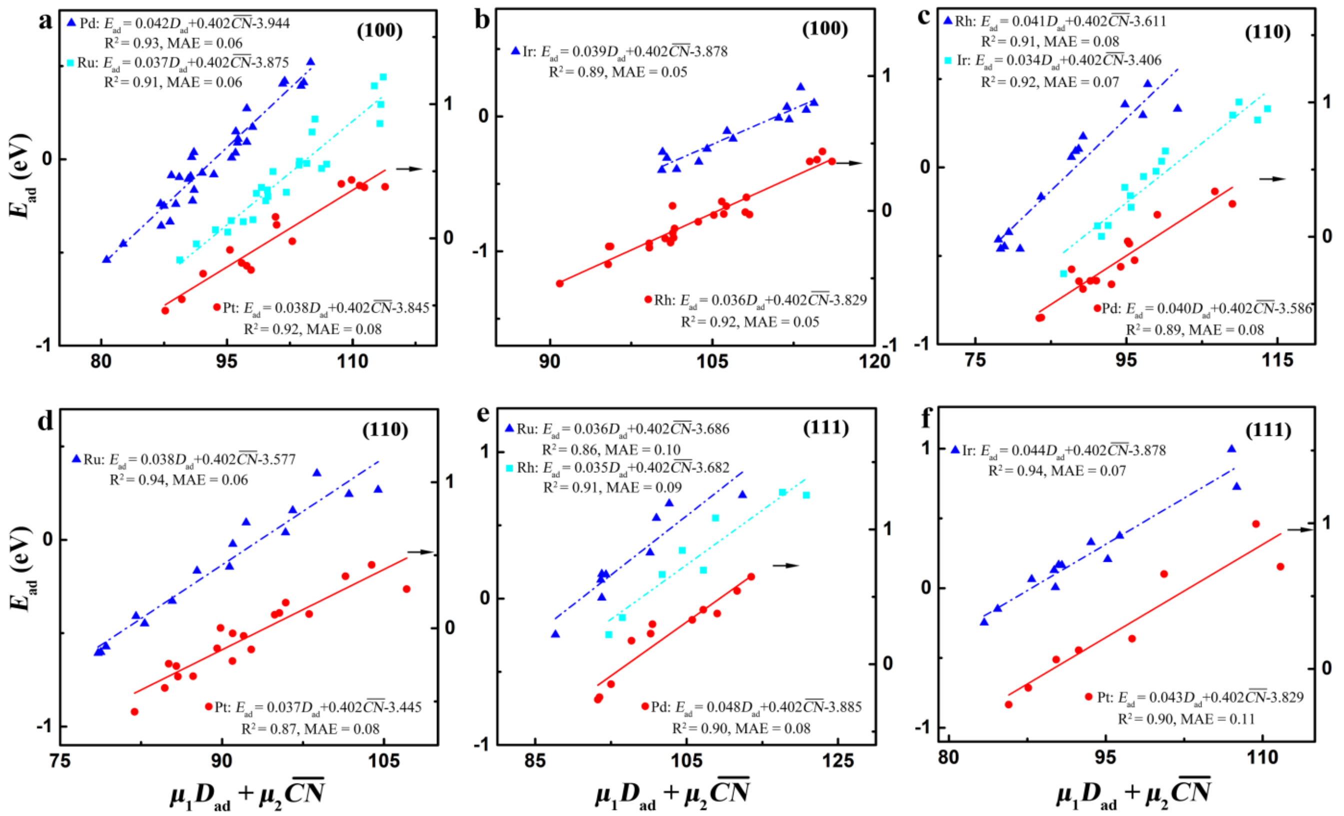


FIG. S25. Adsorption energies of OH against the electronic and geometric descriptors on RuRhIrPdPt-based HEAs with the variable bridge adsorption sites and surrounding environments in both the adsorption-site and environment effects of alloying [5]. (a) and (b), (100) surface with (4 × 4) supercell. (c) and (d), (110) surface with (4 × 4) supercell. (e) and (f), (111) surface with (4 × 4) supercell. All data are calculated by PBE functional. Note that the element symbol in each subfigure denotes that one of the surrounding atoms of adsorption sites is fixed as the corresponding element.

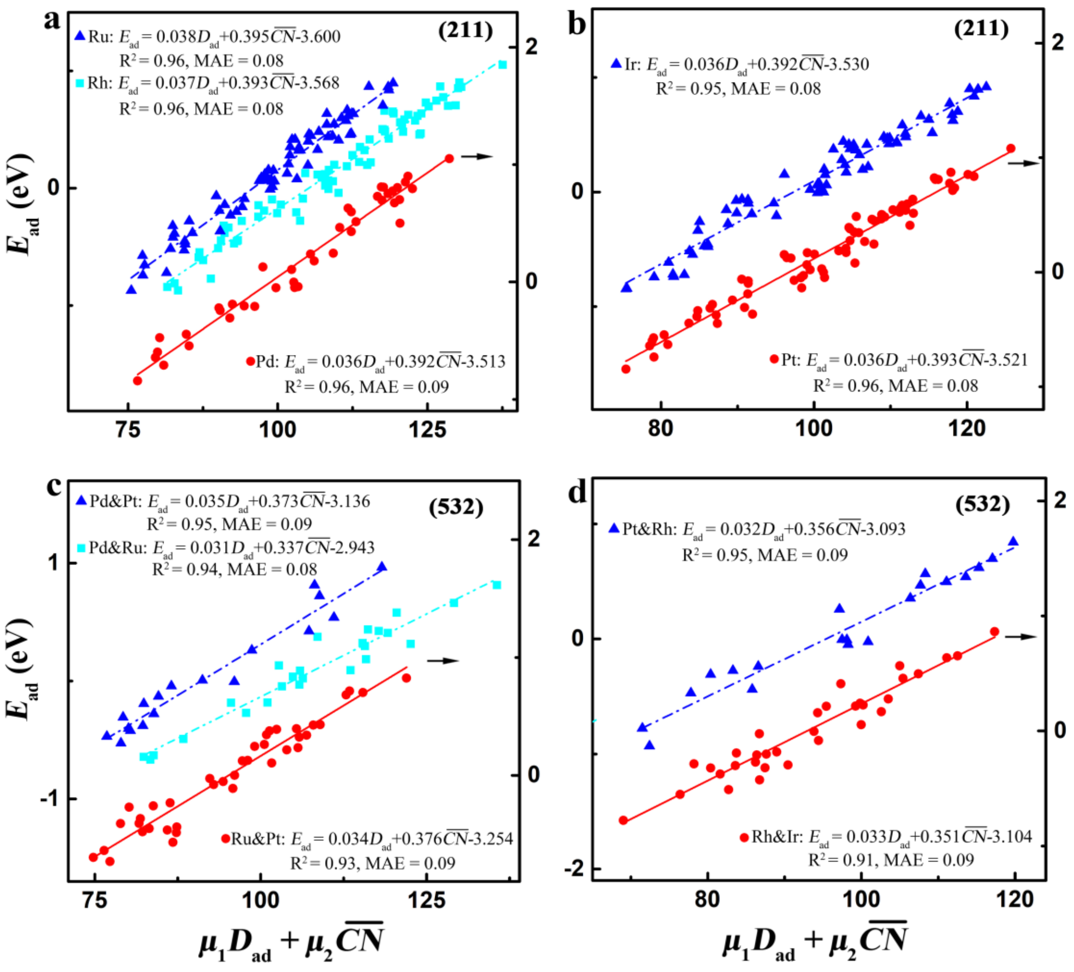


FIG. S26. Adsorption energies of OH against the electronic and geometric descriptors on RuRhIrPdPt-based HEAs with the variable bridge adsorption sites and surrounding environments in both the adsorption-site and environment effects of alloying [5]. (a) and (b), (211) surface with (2 × 4) supercell. (c) and (d), (532) surface with (2 × 2) supercell. All data are calculated by PBE functional. Note that the element symbol in each subfigure denotes that one or two of the surrounding atoms of adsorption sites are fixed as the corresponding element.

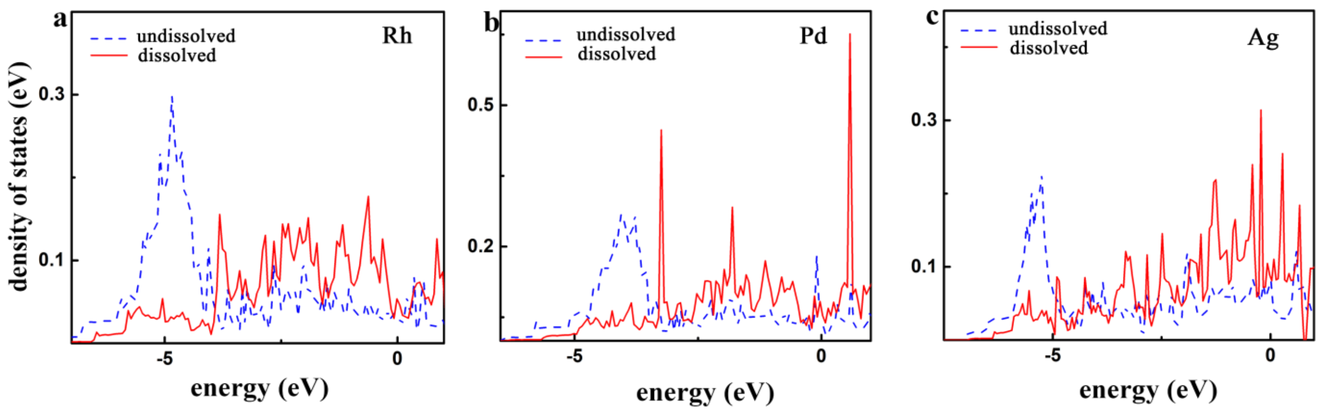


FIG. S27. Density of states of the *s* bands of Rh, Pd and Ag atoms on the undissolved (111) surface and that with three atoms dissolved.

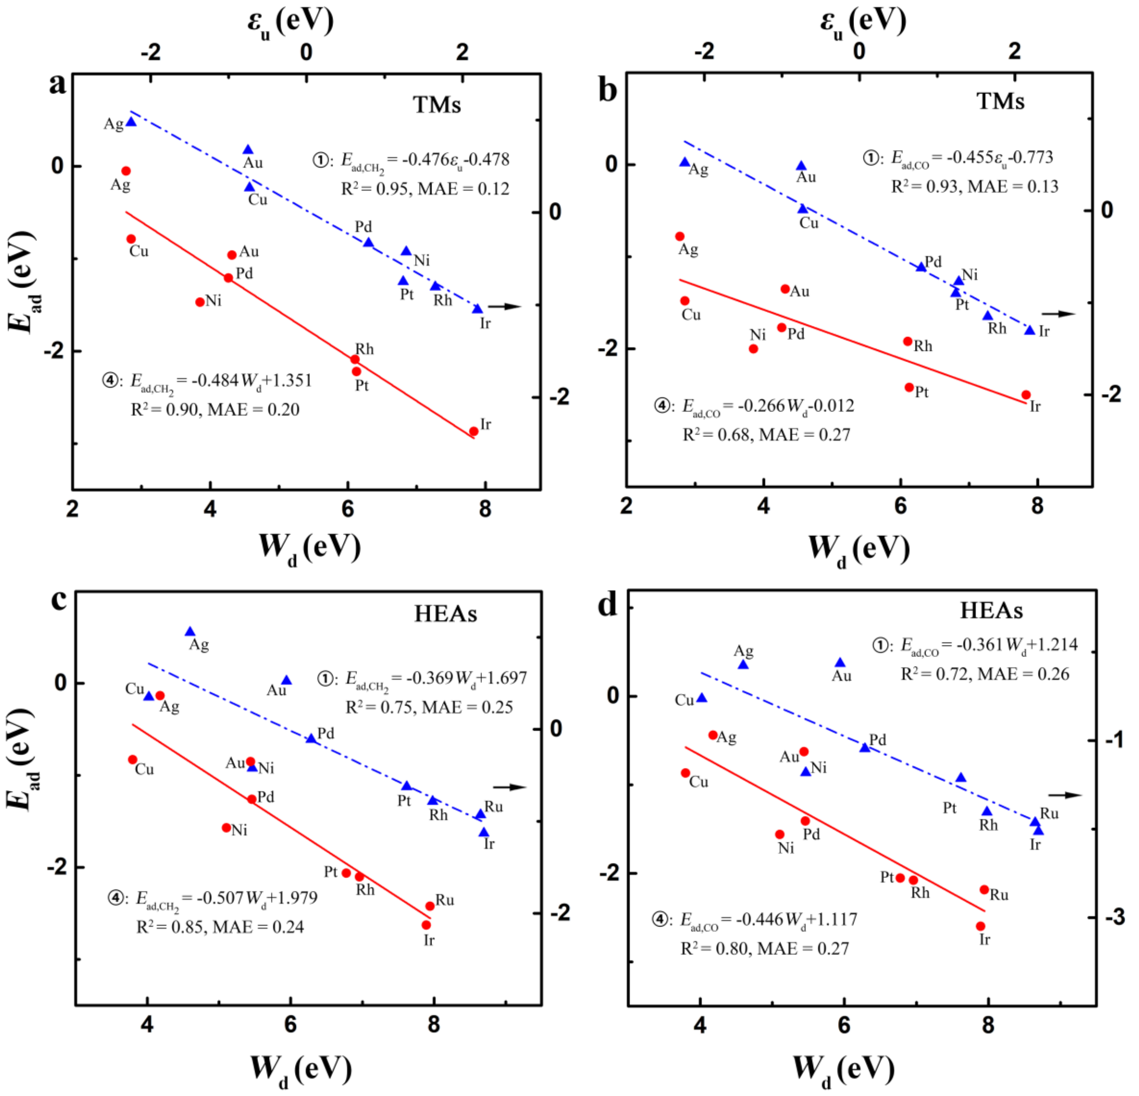


FIG. S28. Adsorption energy of $CH_2$ and CO on (111) surface of TMs (a) and (b) and RuRhIrPdPt-based HEAs (c) and (d) in dissolution against the *d*-band width ($W_d$) and *d*-band upper edge ($\varepsilon_u$). The symbols ① and ④ denote the adsorption on the undissolved surface and that with three atoms dissolved. Note that the CO adsorption on TMs is calculated with RPBE functional [6] while the others are calculated with PBE functional.

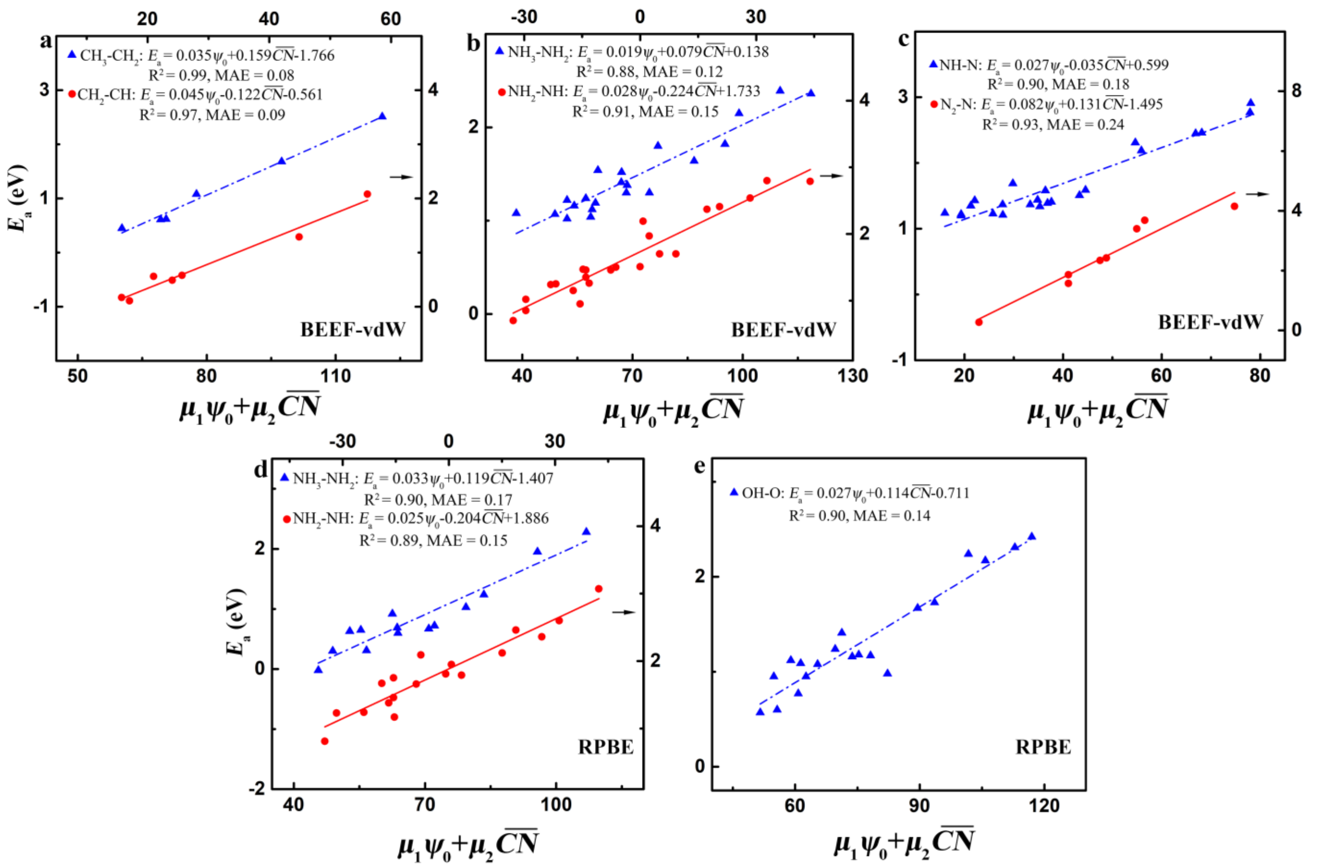


FIG. S29. Activation energies against the electronic and geometric descriptors on TMs. (a), $CH_3 \rightarrow CH_2 + H$ with $CH_3$ at the top site of (111) and (211) surfaces of Ir, Rh, Pt, Cu and Ag TMs and $CH_2 \rightarrow CH + H$ with $CH_2$ at the bridge and fcc sites of (111) and (211) surfaces of Ir, Rh, Pt, Pd, Cu and Ag TMs with the data calculated by BEEF-vdW functional [15]. (b), $NH_3 \rightarrow NH_2 + H$ with $NH_3$ at the top site and $NH_2 \rightarrow NH + H$ with $NH_2$ at the bridge site of close-packed and (211) surfaces of W, Mo, Ir, Pd, Cu, Au, Ni, Ag, Pt, Rh, Os, Ru, Co, and Re TMs with the data calculated by BEEF-vdW functional [15]. (c), $NH \rightarrow N + H$ with NH at the bridge, fcc, hcp and four-fold sites of close-packed and (211) surfaces of Ir, Pd, Cu, Au, Ni, Ag, Pt, Rh, Os, Ru, Co, and Re TMs and $N_2 \rightarrow 2N$ with N at the fcc and hcp sites of close-packed surfaces of W, Cu, Pd, Pt, Ir, Rh, Os and Ru TMs with the data calculated by BEEF-vdW functional [15]. (d), $NH_3 \rightarrow NH_2 + H$ with $NH_3$ at the top site of (111) and (211) surfaces of Ir, Au, Ni, Cu, Re, Ru, Ag, Rh and Pt TMs and $NH_2 \rightarrow NH + H$ with $NH_2$ at the bridge site of (111) surface and (211) surfaces of Cu, Au, Re, Ir, Pt, Ag, Pd, Ru, and Rh TMs with the data calculated by RPBE functional [17]. (e), $OH \rightarrow O + H$ with OH at the fcc site of (111) and (211) surfaces of Cu, Au, Ni, Rh, Ru, Ag, Pd, Pt, Re, Ag, Fe and Ir TMs with the data calculated by RPBE functional [17]. Note that the activation energies on close-packed surfaces and (211) surface calculated by BEEF-vdW functional are modeled with (2 × 2) and (1 × 3) supercells respectively, while those calculated by RPBE functional are modeled with (2 ×2) and (1 ×2) supercells respectively. The close-packed surfaces correspond to fcc(111), bcc(110) and hcp(0001) surfaces. All data are accessible in Ref. [15] at https://www.catalysis-hub.org/energies.

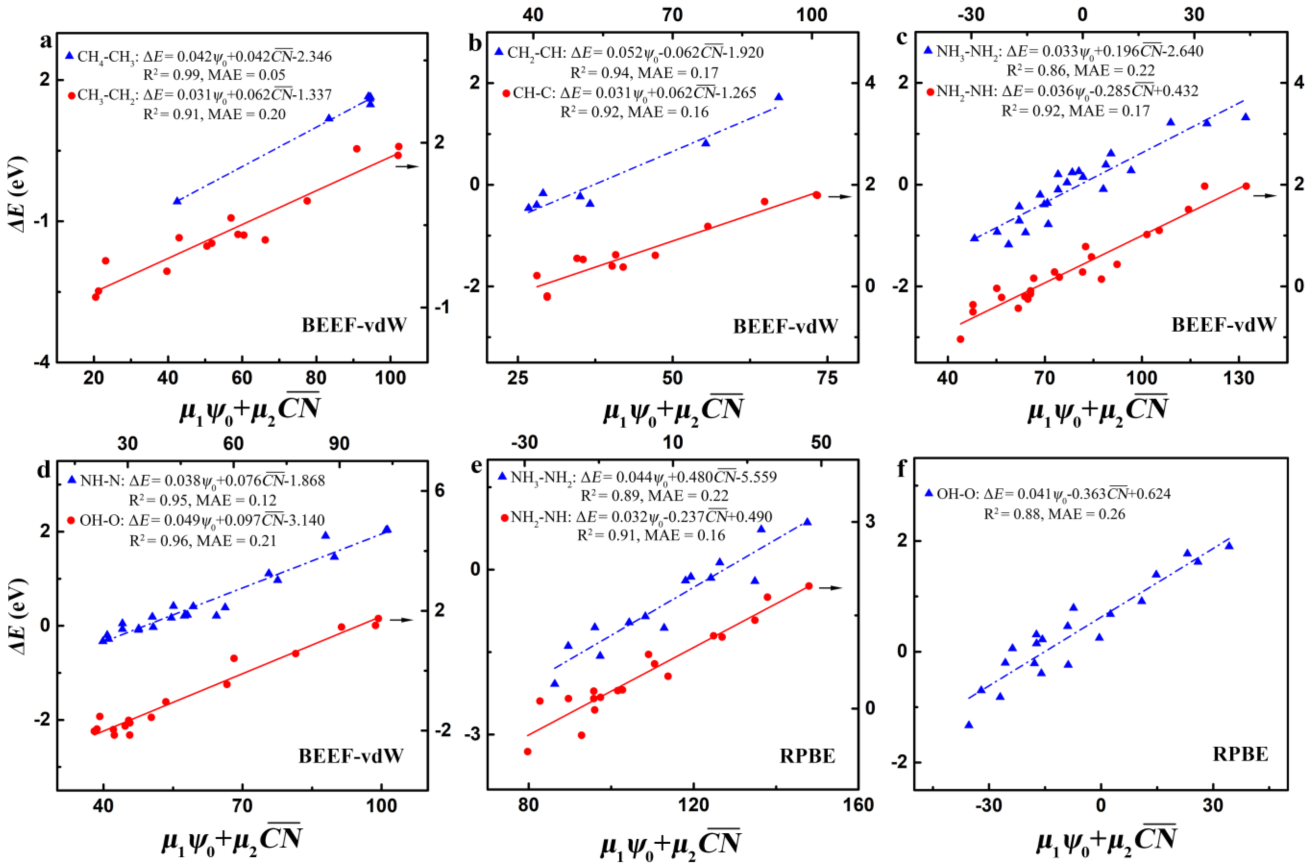


FIG. S30. Reaction energies against the electronic and geometric descriptors on TMs. (a), $CH_4 \rightarrow CH_3 + H$ with $CH_3$ at the top, bridge, fcc and hcp sites of (111) surface of Ag, Au and Fe TMs and $CH_3 \rightarrow CH_2 + H$ with $CH_3$ at the top, fcc and hcp sites of close-packed surfaces of Ag, Au, Ir, Pd, Pt, Rh, Zn, Co, Cu, Ni, Re, Ru, Sc, Y and La TMs with the data calculated by BEEF-vdW functional [15]. (b), $CH_2 \rightarrow CH + H$ with $CH_2$ at the bridge and fcc sites of (111) and (211) surfaces of Rh, Ag, Pd, Ir, Pt and Cu TMs and $CH \rightarrow C + H$ with CH at the fcc and hcp sites of close-packed surfaces of Ag, Au, Co, Cu, Ir, Ni, Os, Pd, Pt, Re, Rh, Ru and Zn TMs with the data calculated by BEEF-vdW functional [15]. (c), $NH_3 \rightarrow NH_2 + H$ with $NH_3$ at the top site of close-packed and (211) surfaces of W, Mo, Ir, Pd, Ag, Pt, Rh, Os, Ru, Co, Re, Cu and Au TMs and $NH_2 \rightarrow NH + H$ with $NH_2$ at the bridge site of close-packed and (211) surfaces of Pt, Au, Cu, Ir, Ni, Pd, Rh, Co, Ru, Os, Re, and Ag TMs with the data calculated by BEEF-vdW functional [15]. (d), $NH \rightarrow N + H$ with NH at the bridge, fcc, hcp and four-fold sites of close-packed and (211) surfaces of Ir, Pd, Cu, Au, Ni, Ag, Pt, Rh, Os, Ru, Co and Re TMs and $OH \rightarrow O + H$ with OH at the bridge, fcc and hcp sites of (111) surface of Pd, Au, Y, La, Sc, Zr, Hf, V, Ag, Ta, Cu, Cd, Tc, Cr, W, Co and Nb TMs with the data calculated by BEEF-vdW functional [15]. (e), $NH_3 \rightarrow NH_2 + H$ with $NH_3$ at the top site of (111) and (211) surfaces of Ir, Rh, Ni, Re, Pt, Au, Cu, Ru and Ag TMs and $NH_2 \rightarrow NH + H$ with $NH_2$ at the bridge site of (111) and (211) surfaces of Cu, Au, Re, Ir, Pt, Ag, Pd, Ru, and Rh TMs with the data calculated by RPBE functional [17]. (e), $OH \rightarrow O + H$ with OH at the fcc site of (111) and (211) surfaces of Cu, Au, Ni, Rh, Ru, Ag, Pd, Pt, Re, Fe and Ir TMs with the data calculated by RPBE functional [17]. Note that the activation energies on close-packed surfaces and (211) surface calculated by BEEF-vdW functional are modeled with (2 × 2) and (1 × 3) supercells respectively, while those calculated by RPBE functional are modeled with (2 × 2) and (1 × 2) supercells respectively. The close-packed surfaces correspond to fcc(111), bcc(110) and hcp(0001) surfaces. All data are accessible in Ref. [15] at https://www.catalysis-hub.org/energies.

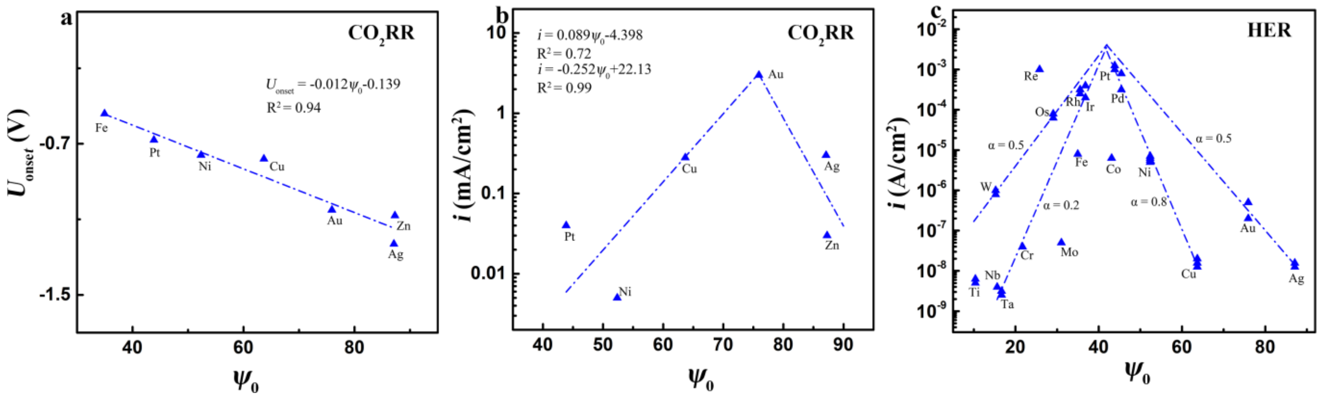


FIG. S31. The activity towards $CO_2$RR and HER against the electronic descriptor on TMs. (a), The experimental onset potential for the overall $CO_2$RR [37,43]. (b), The experimental partial current density for the overall $CO_2$RR at -0.8 V [37,43]. (c), The experimental exchange current density for HER [30,38,44]. α corresponds to the transfer coefficient.

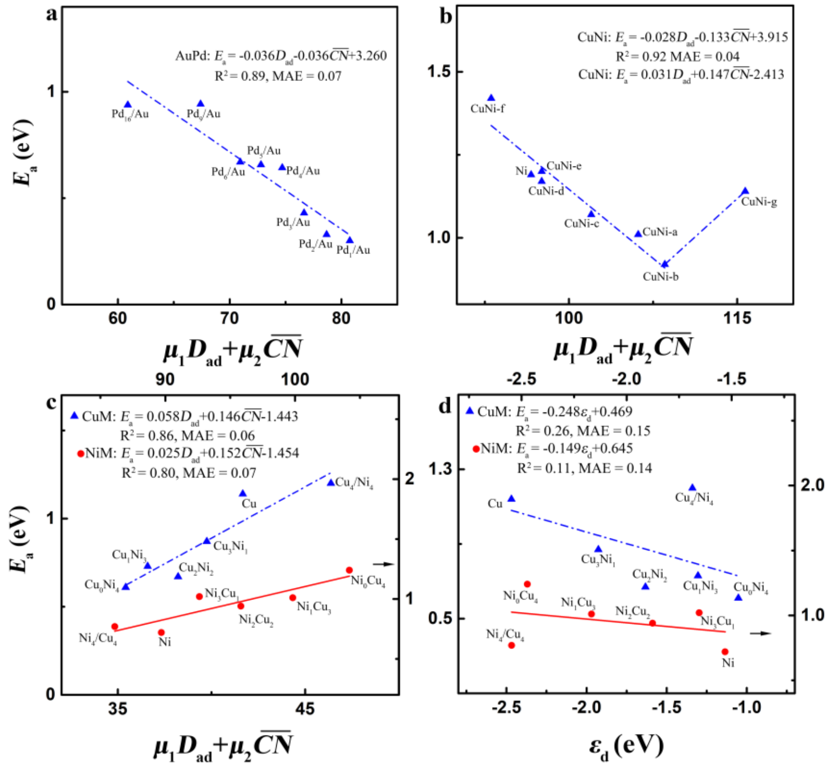


FIG. S32. Activation energies against the electronic and geometric descriptors $D_{ad}$ and $\overline{CN}$ or the *d*-band center ($\varepsilon_d$) on NSAs. (a) Reaction of 2H → $H_2$ with H at the fcc site of (111) surface with (4 × 4) supercell of Au-based AuPd NSAs with the different ratio of Pd ensembles in the topmost layer with the data calculated by PBE functional via van der Waals correction (DFT-D3) [16]. (b), Reaction of OH + H → $H_2O$ with OH+H at the fcc site of (111) surface with (3 × 3) supercell of Ni and Cu-based CuNi NSAs with the different Cu/Ni ratios [including one Ni atom in the topmost layer (CuNi-a), two Ni atoms in the topmost layer (CuNi-c), three Ni atoms in the topmost layer with the different distributions (CuNi-b, CuNi-d and CuNi-e), nine Ni atoms in the topmost layer (CuNi-f), and nine Ni atoms in the subsurface layer (CuNi-g)] with the data calculated by PW91 functional [10]. (c) and (d), Comparison between the electronic and geometric descriptors $D_{ad}$ and $\overline{CN}$ and $\varepsilon_d$ in describing the activation energy of the $H_2O$ → OH + H reaction with OH+H at the fcc+hcp site of (111) surface with (2 × 2) supercell of Cu, Ni, and Cu-based CuNi and Ni-based NiCu NSAs with the different Cu/Ni ratios [including Cu and Ni atoms in the topmost layer ($Cu_xNi_y$ and $Ni_xCu_y$) and Ni ($Cu_4/Ni_4$) or Cu ($Ni_4/Cu_4$) atoms in the subsurface layer] with the data calculated by PBE functional [9].

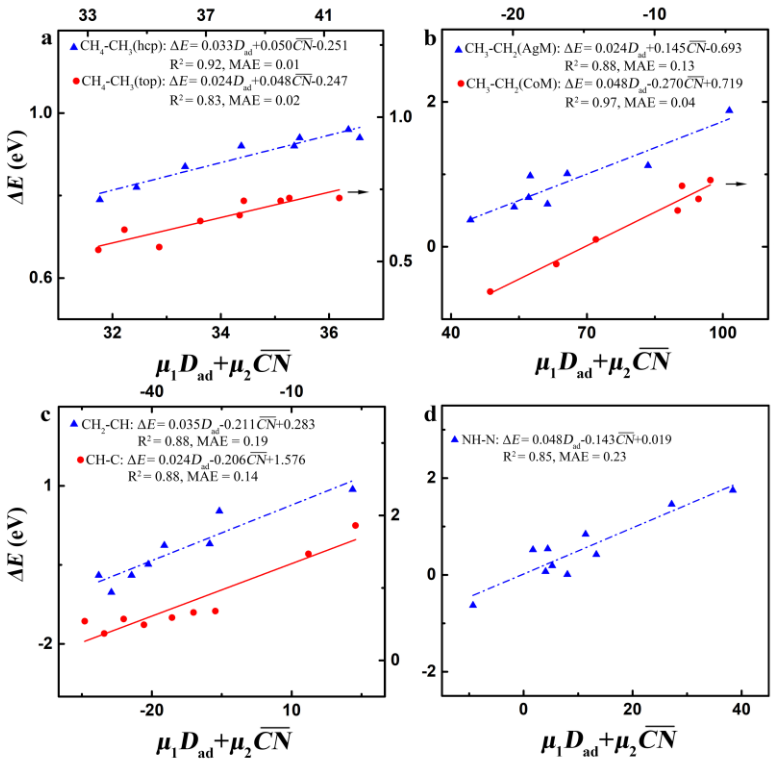


FIG. S33. Reaction energies against the electronic and geometric descriptors on (111) surface of BAs with (2 ×2) supercell [15]. (a), Reaction of $CH_4 \rightarrow CH_3 + H$ with $CH_3$ at the top and hcp sites of Os-based $Os_3M$ (M = Ag, Au, Co, Cu, Ir, Ni, Pt, Rh, and Ru) BAs. (b), Reaction of $CH_3 \rightarrow CH_2 + H$ with $CH_3$ at the top, bridge, fcc and hcp sites of Ag-based AgM (M = Au, Cu, Fe, Ir, Os, Pt, Rh, and Ru) and Co-based CoM (M = Cu, Ir, Os, Ni, Pt, Pd and Ru) BAs. (c), Reaction of $CH_2 \rightarrow CH + H$ with $CH_2$ at the top, bridge, and hcp sites of Ag-based AgM (M = Au, Cu, Ir, Ni, Os, Pt, Pd, and Ru) and $CH \rightarrow C + H$ with CH at the bridge, fcc and hcp sites of Ag-based AgM (M = Au, Cu, Fe, Ir, Ni, Pt, Pd, Rh and Ru) BAs. (d), Reaction of $NH \rightarrow N + H$ with NH at the top, bridge, fcc and hcp sites of Ag-based AgM (M = Au, Cu, Co, Ir, Ni, Os, Pt, Pd, Rh and Ru) BAs. All data are calculated with BEEF-vdW functional. Note that all data are accessible in Ref. [15] at https://www.catalysis-hub.org/energies.

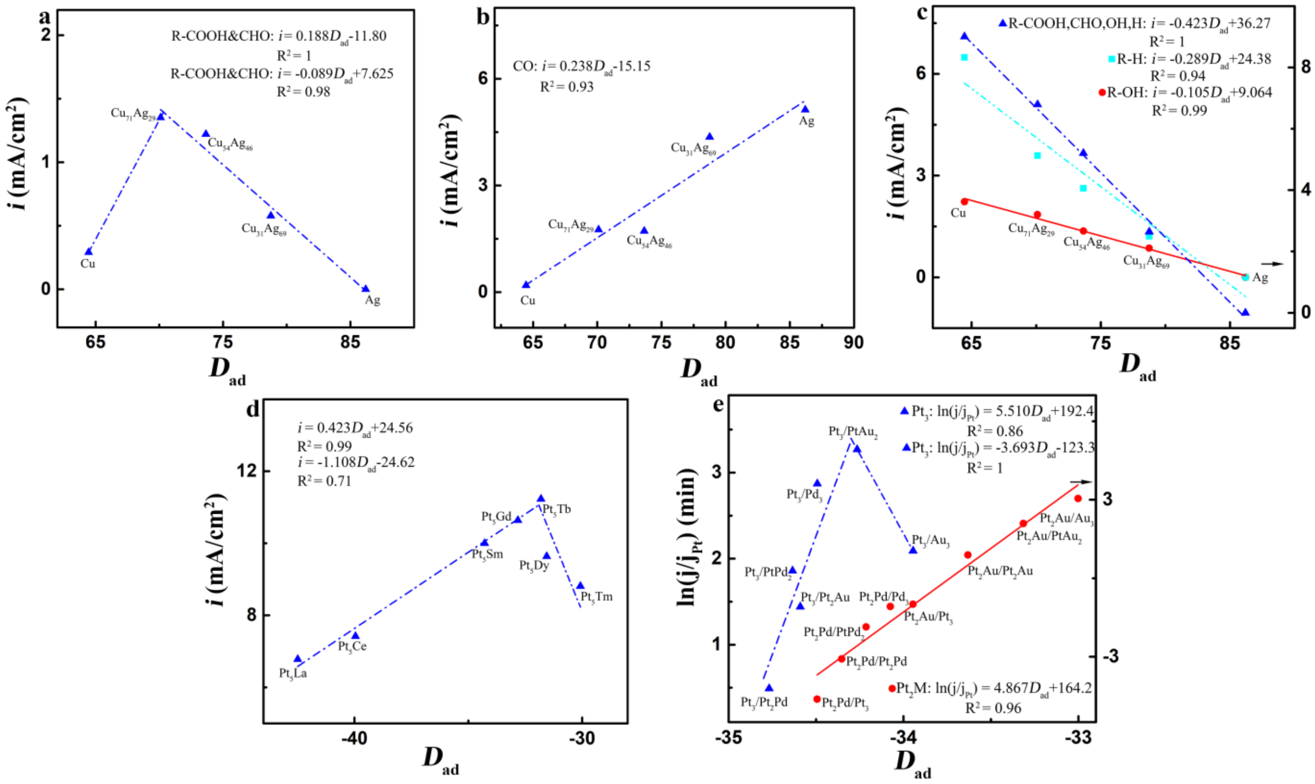


FIG. S34. The activity towards $CO_2$RR and ORR against the electronic descriptor on BAs and NSAs. (a)-(c), The experimental partial current density for the R-COOH, R-CHO, CO, R-H and R-OH production towards $CO_2$RR at -1.05 V vs. RHE on Cu, Ag, and $Cu_{31}Ag_{69}$, $Cu_{54}Ag_{46}$, and $Cu_{71}Ag_{29}$ BAs. R-X denotes the product that containing the X-group (COOH, CHO, H and OH) during the $CO_2$RR process [35]. (d), The experimental kinetic current density towards ORR at 0.9 V vs. RHE on La-series $Pt_5M$ BAs. Note that the 4*f*-, 5*d*- and 6*s*-electrons of La-series metals are considered as valence electrons [39]. (e), The DFT-calculated activity towards ORR on Pt-based NSAs with $A_xB_{3-x}/A_yB_{3-y}$ monolayers. $A_xB_{3-x}$($A_yB_{3-y}$) corresponds to the first (second) layer on Pt(111) host and the subscripts $x$ and $y$ denote the stoichiometry of the corresponding atoms [36].

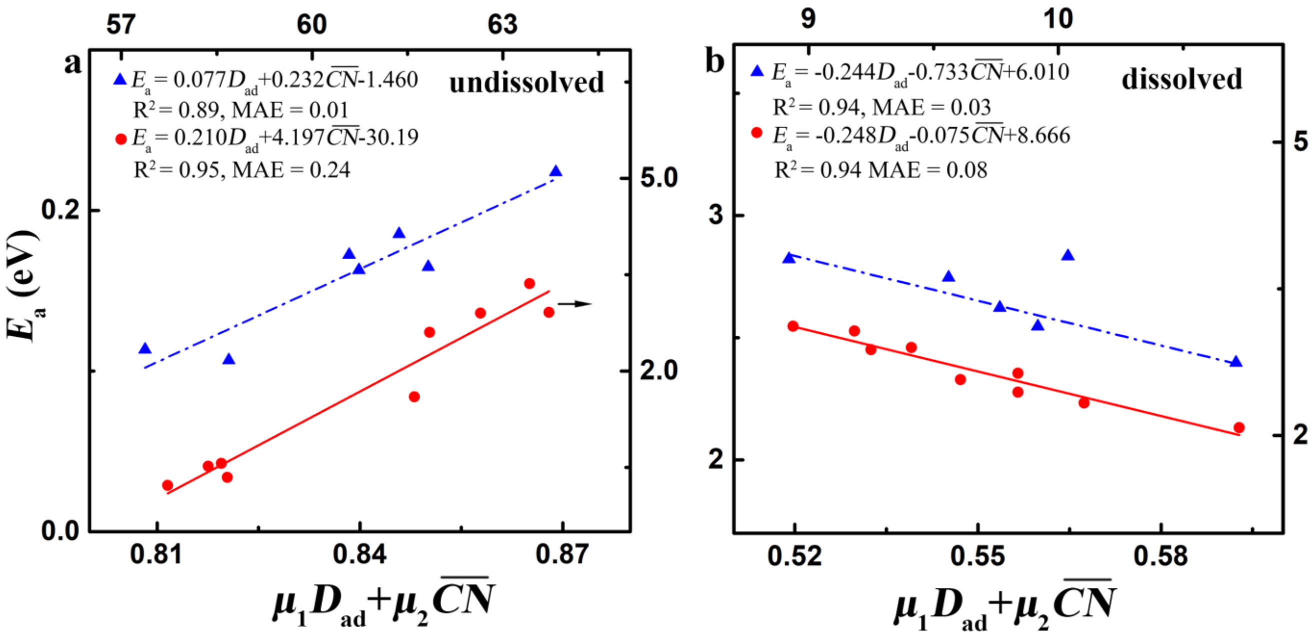


FIG. S35. Activation energies of $CH_2 \rightarrow CH + H$ reaction against the electronic and geometric descriptors on (111) surface of RuRhIrPdPt-based HEAs with (4 × 4) supercell. (a), Undissolved (111) surface. (b) (111) surface with three atoms dissolved. The blue triangle denotes the adsorption-site effect of alloying while the red circle does both the adsorption-site and environment effects of alloying. All data are calculated with PBE functional.

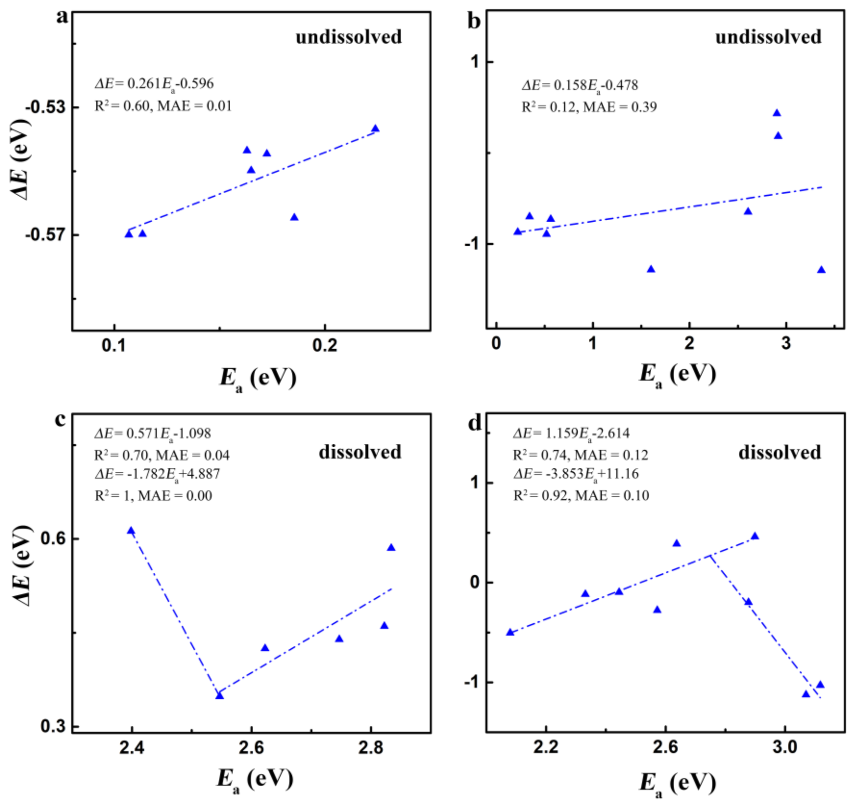


FIG. S36. BEP relation of $CH_2 \rightarrow CH + H$ reaction on (111) surface of RuRhIrPdPt-based HEAs with (4 × 4) supercell. (a), Undissolved (111) surface in the adsorption-site effect of alloying. (b), Undissolved (111) surface in both the adsorption-site and environment effects of alloying. (c), (111) surface with three atoms dissolved in the adsorption-site effect of alloying. (d), (111) surface with three atoms dissolved in both the adsorption-site and environment effects of alloying. All data are calculated with PBE functional.

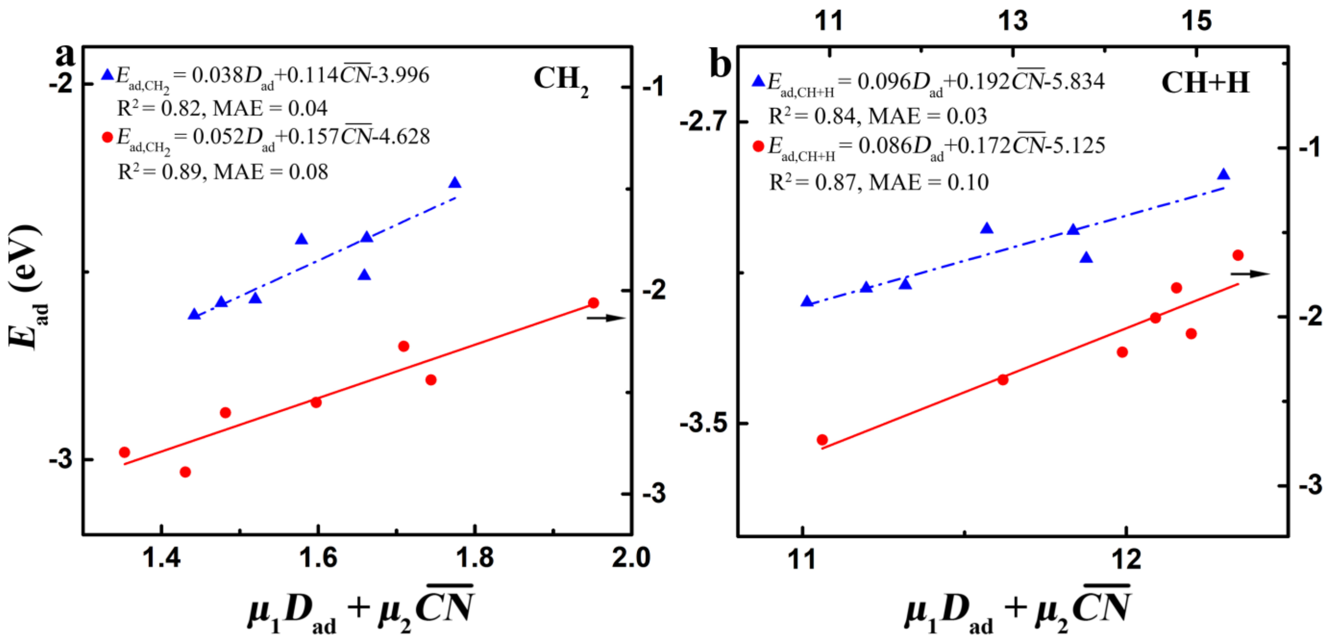


FIG. S37. Adsorption energies of $CH_2$ and CH+H against the electronic and geometric descriptors on RuRhIrPdPt-based HEAs in the adsorption-site effect of alloying. (a), $CH_2$ adsorption at the hcp site of the undissolved (111) surface (blue triangle) and the bridge site of (111) surface with three atoms dissolved (red circle). (b), CH and H coadsorption on the undissolved (111) surface (blue triangle) and (111) surface with three atoms dissolved (red circle). All data are calculated with PBE functional.

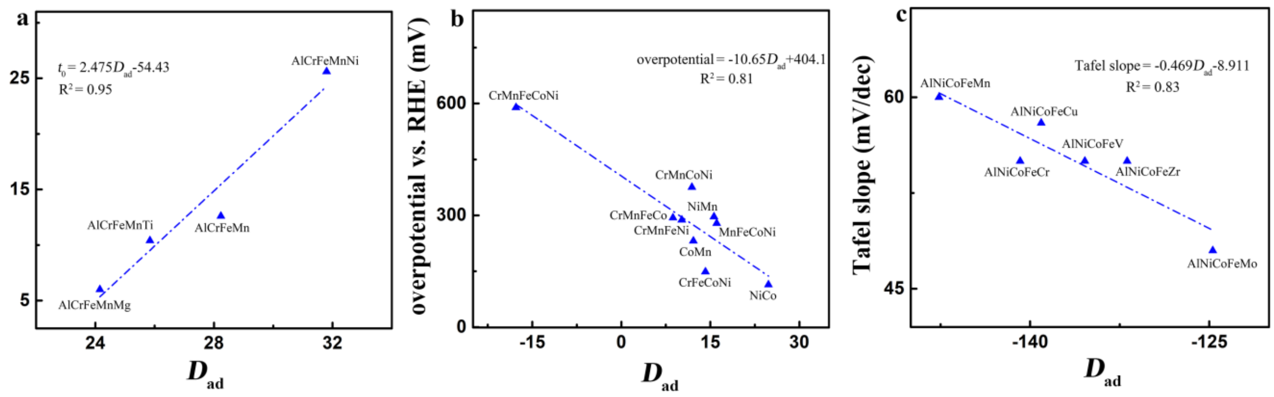


FIG. S38. The activity against the electronic descriptor on HEAs. (a), The experimental decoloration time ($t_0$) of decolorization reaction (corresponding to the reaction efficiency) on AlCrFeMn-based HEAs [31]. (b), The experimental overpotential at −0.5 V towards ORR on HEAs and BAs [34]. (c), The experimental Tafel slopes towards OER on AlNiCoFe-based HEAs [32].

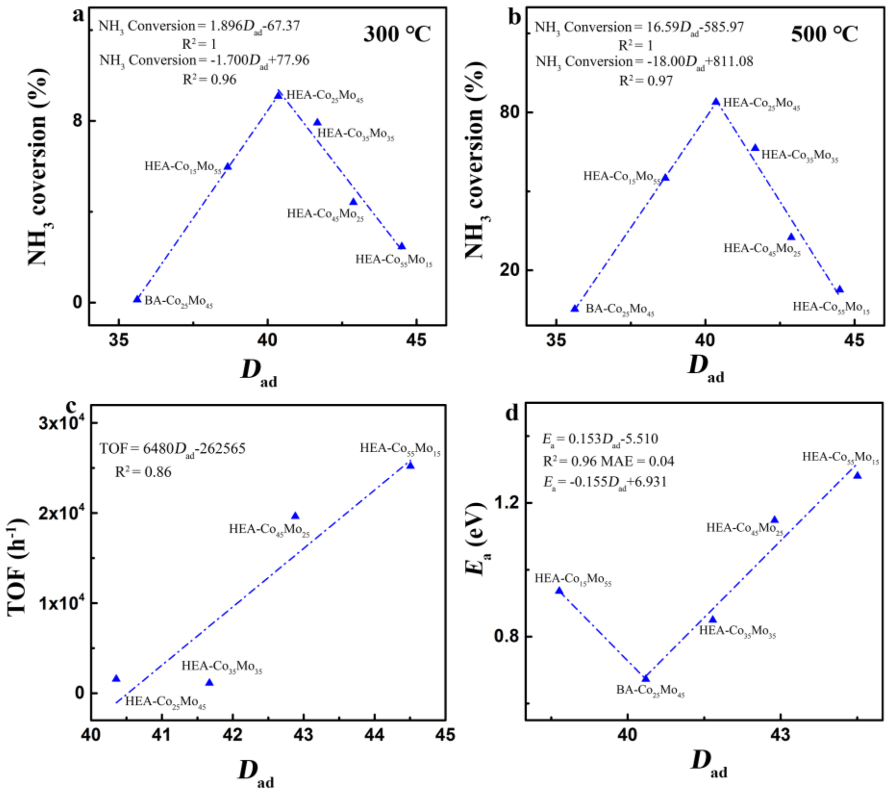


FIG. S39. The activity towards ammonia decomposition against the electronic descriptor on HEAs [33]. (a) and (b), The experimental $NH_3$ conversion efficiency under the different reaction temperatures 300°C and 500°C on HEAs (HEA-Co$_x$Mo$_y$) and BAs (BA-Co$_x$Mo$_y$) with the different Co/Mo ratios. (c), The experimental turnover frequency (TOF) on HEAs with the different Co/Mo ratios. (d), The experimental-estimated activation energy on HEAs with the different Co/Mo ratios.

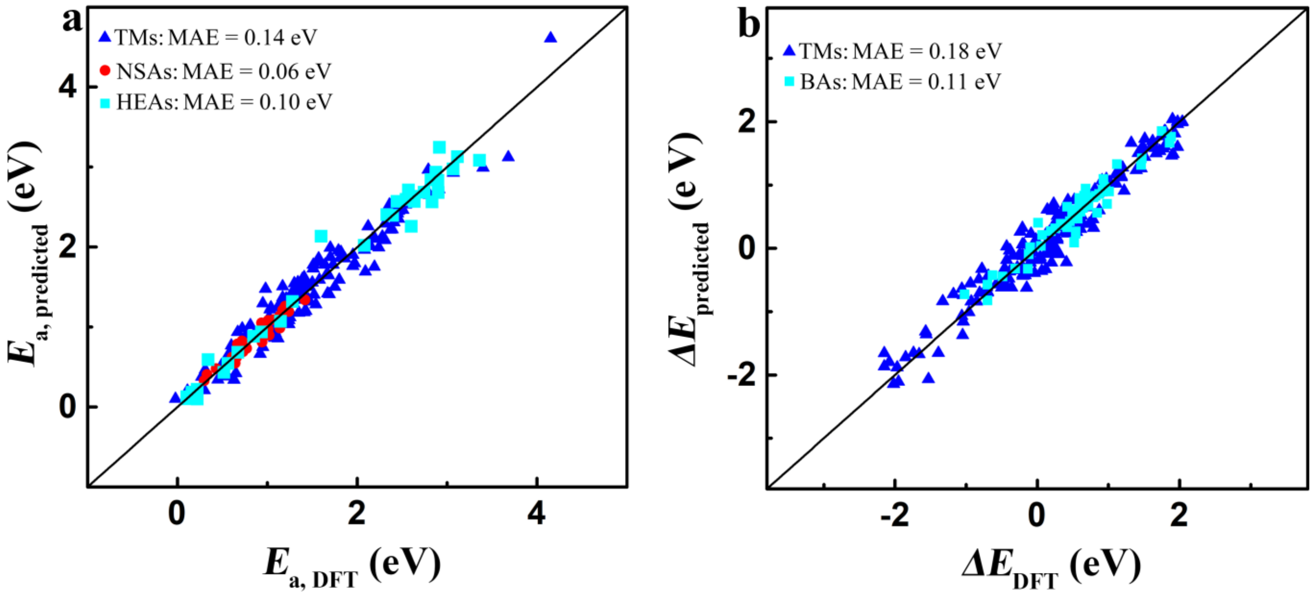


FIG. S40. Comparison between the predicted and DFT-calculated activation energies ($E_a$) and reaction energies ($\Delta E$) on TMs, NSAs, BAs and HEAs [9,10,15–17].

Table S1. Comparison between the predicted prefactors of $D_{ad}$ and $\overline{CN}$ terms $\mu_1$ and $\mu_2$ in Eq. (2) in the main text and the DFT-calculated ones for the different adsorbates at the various adsorption sites of TMs [7]. Columns 2 and 3 show the predicted ones while Columns 4-11 show the fitted results shown in Figs. S13c-f.

| **species** | **Predicted** | | **TMs** | | | | | | | |
|---|---|---|---|---|---|---|---|---|---|---|
| | | | **(100)** | | **(111)** | | **(211)** | | | |
| | | | hollow | | hcp | | hcp | | four-fold | |
| | $\mu_1$ | $\mu_2$ | $\mu_1$ | $\mu_2$ | $\mu_1$ | $\mu_2$ | $\mu_1$ | $\mu_2$ | $\mu_1$ | $\mu_2$ |
| CH | 0.060 | 0.080 | 0.062 | 0.080 | 0.068 | 0.082 | 0.063 | 0.082 | 0.058 | 0.075 |
| **species** | **Predicted** | | **(100)** | | **(110)** | | **(211)** | | | |
| | | | bridge | | top | | top | | bridge | |
| | $\mu_1$ | $\mu_2$ | $\mu_1$ | $\mu_2$ | $\mu_1$ | $\mu_2$ | $\mu_1$ | $\mu_2$ | $\mu_1$ | $\mu_2$ |
| CO | 0.040 | 0.120 | 0.037 | 0.110 | 0.033 | 0.114 | 0.033 | 0.117 | 0.038 | 0.114 |

Table S2. Comparison between the predicted prefactors of $D_{\mathrm{ad}}$ and $\overline{CN}$ terms $\mu_1$ and $\mu_2$ in Eq. (2) in the main text and the DFT-calculated ones for $NH_2$ and OH at the top site of (100) surface of Ag-based AgM BAs in the adsorption-site effect of alloying, for C, CH and CO at the bridge, fcc, hcp and four-fold sites of (211) surface of AgAu, AgPd, IrRu, and PtRh BAs [7] in both the adsorption-site and environment effects of alloying, and for OH at the hcp site of (111) surface of Ag-based $Ag_3M$ BAs [15] in both the adsorption-site and environment effects of alloying. Columns 2 and 3 show the predicted ones while Columns 4-13 show the fitted results shown in Fig. 2f in the main text and Figs. S20, S23 and S24a. Note that the adsorption energies of OH at the hcp site of (111) surface of Ag-based $Ag_3M$ BAs are obtained on fixed surface sites, thus the prefactor of $\mu_2$ is not fitted as $\overline{CN}$ of the adsorption site is unchanged.

| **species** | **predicted** | | **BAs** | | | | | | | | | |
|---|---|---|---|---|---|---|---|---|---|---|---|---|
| | | | **top** | | **bridge** | | **fcc** | | **hcp** | | **four-fold** | |
| | $\mu_1$ | $\mu_2$ | $\mu_1$ | $\mu_2$ | $\mu_1$ | $\mu_2$ | $\mu_1$ | $\mu_2$ | $\mu_1$ | $\mu_2$ | | |
| C | 0.080 | 0.040 | | | | | | | 0.064 | 0.041 | 0.065 | 0.042 |
| CH | 0.060 | 0.080 | | | 0.066 | 0.079 | 0.051 | 0.072 | 0.056 | 0.079 | 0.054 | 0.076 |
| CO | 0.040 | 0.120 | | | 0.034 | 0.119 | | | | | | |
| $NH_2$ | 0.025 | 0.150 | 0.026 | 0.105 | | | | | | | | |
| OH | 0.033 | 0.134 | 0.023 | 0.168 | | | | | 0.026 | | | |

Table S3. Comparison between the predicted prefactors of $D_{ad}$ and $\overline{CN}$ terms $\mu_1$ and $\mu_2$ in Eq. (2) in the main text and the DFT-calculated ones for $NH_2$ and OH at the top site of (111) surface of Cu-based NSAs in the adsorption-site effect of alloying, for $CH_x$ ($x$ = 0-3), CO, $NH_x$ ($x$ = 0-2), OH, F, and Cl at the top site of (111) and (100) surfaces of Pt(Pd)-based NSAs [11–14] in the environment effect of alloying, and for OH at the fcc site of (111) surface of Cu-based or Ni-based CuNi NSAs with the different Cu/Ni ratios [9,10] in both the adsorption-site and environment effects of alloying. Columns 2 and 3 show the predicted ones while Columns 4-11 show the fitted results shown in Figs. S20, S22, and S24b-e. Note that the adsorption energies on NSAs in the environment effect of alloying and in both the adsorption-site and environment effects of alloying are obtained on fixed surface sites, thus the prefactor of $\mu_2$ is not fitted as $\overline{CN}$ of the adsorption site is unchanged.

| **species** | **predicted** | | **adsorption-site effect of alloying** | | | | | | | |
|---|---|---|---|---|---|---|---|---|---|---|
| | $\mu_1$ | $\mu_2$ | $\mu_1$ | $\mu_2$ | | | | | | |
| $NH_2$ | 0.025 | 0.150 | 0.021 | 0.141 | | | | | | |
| OH | 0.033 | 0.134 | 0.018 | 0.138 | | | | | | |
| **species** | **predicted** | | **environment effect of alloying** | | | | | | | |
| | | | **I** [11] | | **II** [14] | | **III** [13] | | **IV** [12] | |
| | $\mu_1$ | $\mu_2$ | $\mu_1$ | $\mu_2$ | $\mu_1$ | $\mu_2$ | $\mu_1$ | $\mu_2$ | $\mu_1$ | $\mu_2$ |
| C | 0.080 | 0.040 | 0.086 | | | | | | | |
| CH | 0.060 | 0.080 | 0.085 | | | | | | | |
| $CH_2$ | 0.040 | 0.120 | 0.038 | | | | | | | |
| $CH_3$ | 0.020 | 0.160 | 0.028 | | | | | | | |
| CO | 0.040 | 0.120 | 0.044 | | 0.035/0.040 | | | | | |
| N | 0.075 | 0.050 | 0.076 | | | | | | | |
| NH | 0.050 | 0.100 | 0.066 | | | | | | | |
| $NH_2$ | 0.025 | 0.150 | 0.023 | | | | | | | |
| OH | 0.033 | 0.134 | | | | | 0.033 | | | |
| F | 0.050 | 0.100 | | | | | | | 0.055 | |
| Cl | 0.050 | 0.100 | | | | | | | 0.049 | |
| **species** | **predicted** | | **adsorption-site and environment effects of alloying** | | | | | | | |
| | | | **I** [10] | | **II** [9] | | **III** [9] | | | |
| | | | **Cu-based** | | **Cu-based** | | **Ni-based** | | | |
| | $\mu_1$ | $\mu_2$ | $\mu_1$ | $\mu_2$ | $\mu_1$ | $\mu_2$ | $\mu_1$ | $\mu_2$ | | |
| OH | 0.033 | 0.134 | 0.033 | | 0.032 | | 0.034 | | | |

Table S4. The coefficients $k_1$ and $k_2$ in Eq. (4) in the main text for the adsorption energy on NSAs, BAs, and HEAs in the adsorption-site and environment effects of alloying. Rows 1 and 2 show the coefficients $k_1$ and $k_2$ of the adsorption energy of $CH_x$ ($x$ = 1-3), CO, $NH_x$ ($x$ = 1, 2), and OH on Cu-based NSAs, Ag-based BAs, and RuRhIrPdPt-based HEAs in the adsorption-site effect of alloying (Fig. 2c-e and Figs. S14b, S20 and S21). Rows 3-14 show the coefficients $k_1$ and $k_2$ of the adsorption energy of $CH_2$ and CO on Ru(Cu)RhIrPdPt-based HEAs, OH on Ag-based BAs, and $CH_x$ ($x$ = 0-3), CO, $NH_x$ ($x$ = 0-2), OH, F, and Cl on Pt(Pd)-based NSAs [11–14] in the environment effect of alloying (Fig. 2c and d and Fig. S22), while Rows 15-20 show the coefficients $k_1$ and $k_2$ of the adsorption energy of OH on RuRhIrPdPt-based HEAs [5], C, CH and CO on AgAu, AgPd, IrRu, PtRh [7] BAs, OH on Ag-based $Ag_3M$ BAs [15], and OH, H and OH+H on Cu(Ni)-based NSAs [9,10] in both the adsorption-site and environment effects of alloying (Fig. 2f and Figs. S23-S26).

| | | | | | | | | | | | |
|---|---|---|---|---|---|---|---|---|---|---|---|
| **adsorption-site effect on NSAs, BAs, and HEAs** | **all considered adsorbates** | $k_1$ | $k_2$ | | | | | | | | |
| | | 0.10 | 0.90 | | | | | | | | |
| **environment effect** | **$CH_2$ on HEAs** | **Ru** | | **Rh** | | **Ir** | | **Pd** | | **Pt** | |
| | | $k_1$ | $k_2$ | $k_1$ | $k_2$ | $k_1$ | $k_2$ | $k_1$ | $k_2$ | $k_1$ | $k_2$ |
| | | 0.54 | 0.80 | 1.22 | 0.10 | 3.68 | -4.60 | 2.12 | -0.80 | 0.45 | 0.50 |
| | **CO on HEAs** | **Ru** | | **Cu** | | | | | | | |
| | | $k_1$ | $k_2$ | $k_1$ | $k_2$ | | | | | | |
| | | 2.08 | -0.35 | 0.01 | 1.00 | | | | | | |
| | **OH on BAs** | $k_1$ | $k_2$ | | | | | | | | |
| | | -0.08 | 1.22 | | | | | | | | |
| | **NSAs** | **Pt-based** | | **Pt-based** | | **Pt-based** | | **Pt-based** | | **Pd-based** | |
| | | $CH_x$ ($x$ = 0-3) and $NH_x$ ($x$ = 0-2) | | CO | | OH | | F and Cl | | CO | |
| | | $k_1$ | $k_2$ | $k_1$ | $k_2$ | $k_1$ | $k_2$ | $k_1$ | $k_2$ | $k_1$ | $k_2$ |
| | | -0.65 | 1.00 | -0.50 | 1.00 | -1.36 | 1.00 | -1.00 | 1.00 | -0.36 | 1.00 |
| **adsorption-site and environment effects** | **OH on HEAs** | $k_1$ | $k_2$ | | | | | | | | |
| | | 0.90 | -0.10 | | | | | | | | |
| | **C, CH, CO and OH on BAs** | $k_1$ | $k_2$ | | | | | | | | |
| | | 1.00 | 0.10 | | | | | | | | |
| | **OH, H and OH+H on NSAs** | $k_1$ | $k_2$ | | | | | | | | |
| | | 0.28 | 0.34 | | | | | | | | |

Table S5. Comparison between the predicted prefactors of $D_{ad}$ and $\overline{CN}$ terms $\mu_1$ and $\mu_2$ in Eq. (2) in the main text and the DFT-calculated ones for OH adsorption at the bridge site of RuRhIrPdPt-based HEAs. Columns 2 and 3 show the predicted ones while Columns 4-15 show the fitted results shown in Fig. 2f in the main text and Fig. S25. Note that the adsorption energies of OH on undissolved surfaces of HEAs are extracted from Ref. [5].

| species | **predicted** | | **undissolved (111) surface** | | | | | | | | | | **dissolved (111) surface** | |
|---|---|---|---|---|---|---|---|---|---|---|---|---|---|---|
| | | | fixing Ru | | fixing Rh | | fixing Ir | | fixing Pd | | fixing Pt | | | |
| | $\mu_1$ | $\mu_2$ | $\mu_1$ | $\mu_2$ | $\mu_1$ | $\mu_2$ | $\mu_1$ | $\mu_2$ | $\mu_1$ | $\mu_2$ | $\mu_1$ | $\mu_2$ | $\mu_1$ | $\mu_2$ |
| **OH** | 0.033 | 0.402 | 0.036 | 0.402 | 0.035 | 0.402 | 0.044 | 0.402 | 0.048 | 0.402 | 0.043 | 0.402 | 0.040 | 0.519 |

Table S6. Comparison between the predicted prefactors of $D_{ad}$ and $\overline{CN}$ terms $\mu_1$ and $\mu_2$ in Eq. (2) in the main text and the DFT-calculated ones for OH adsorption at the bridge site of RuRhIrPdPt-based HEAs [5]. Columns 2 and 3 show the predicted ones while Columns 4-13 show the fitted results shown in Figs. S25 and S26.

| **species** | **predicted** | | **(100) surface** | | | | | | | | | |
|---|---|---|---|---|---|---|---|---|---|---|---|---|
| | | | fixing Ru | | fixing Rh | | fixing Ir | | fixing Pd | | fixing Pt | |
| | $\mu_1$ | $\mu_2$ | $\mu_1$ | $\mu_2$ | $\mu_1$ | $\mu_2$ | $\mu_1$ | $\mu_2$ | $\mu_1$ | $\mu_2$ | $\mu_1$ | $\mu_2$ |
| OH | 0.033 | 0.402 | 0.037 | 0.402 | 0.036 | 0.402 | 0.039 | 0.402 | 0.042 | 0.402 | 0.038 | 0.402 |
| **species** | **predicted** | | **(110) surface** | | | | | | | | | |
| | | | fixing Ru | | fixing Rh | | fixing Ir | | fixing Pd | | fixing Pt | |
| | $\mu_1$ | $\mu_2$ | $\mu_1$ | $\mu_2$ | $\mu_1$ | $\mu_2$ | $\mu_1$ | $\mu_2$ | $\mu_1$ | $\mu_2$ | $\mu_1$ | $\mu_2$ |
| OH | 0.033 | 0.402 | 0.038 | 0.402 | 0.041 | 0.402 | 0.034 | 0.402 | 0.040 | 0.402 | 0.037 | 0.402 |
| **species** | **predicted** | | **(211) surface** | | | | | | | | | |
| | | | fixing Ru | | fixing Rh | | fixing Ir | | fixing Pd | | fixing Pt | |
| | $\mu_1$ | $\mu_2$ | $\mu_1$ | $\mu_2$ | $\mu_1$ | $\mu_2$ | $\mu_1$ | $\mu_2$ | $\mu_1$ | $\mu_2$ | $\mu_1$ | $\mu_2$ |
| OH | 0.033 | 0.402 | 0.038 | 0.395 | 0.037 | 0.393 | 0.036 | 0.392 | 0.036 | 0.392 | 0.036 | 0.393 |
| **species** | **predicted** | | **(532) surface** | | | | | | | | | |
| | | | fixing Ru&Pt | | fixing Pd&Pt | | fixing Pd&Ru | | fixing Pt&Rh | | fixing Rh&Ir | |
| | $\mu_1$ | $\mu_2$ | $\mu_1$ | $\mu_2$ | $\mu_1$ | $\mu_2$ | $\mu_1$ | $\mu_2$ | $\mu_1$ | $\mu_2$ | $\mu_1$ | $\mu_2$ |
| OH | 0.033 | 0.402 | 0.034 | 0.376 | 0.035 | 0.373 | 0.031 | 0.337 | 0.032 | 0.356 | 0.033 | 0.351 |

Table S7. Comparison between the accuracy of Eqs. (2-4) in the main text by introducing the cohesive energy and the *d*-band width of the adsorption-sites' TM atoms in predicting the adsorption energy on TMs, NSAs, BAs, and HEAs in the adsorption-site effect of alloying in dissolution. MAE: mean absolute error.

| | **MAE (eV)** | |
|---|---|---|
| | **Cohesive energy** | ***d*-band width** |
| **TMs** | 0.16 | 0.32 |
| **NSAs** | 0.23 | 0.34 |
| **BAs** | 0.14 | 0.38 |
| **HEAs** | 0.19 | 0.41 |

References


[1] G. Kresse and J. Furthmüller, *Efficient Iterative Schemes for Ab Initio Total-Energy Calculations Using a Plane-Wave Basis Set*, Phys. Rev. B **54**, 11169 (1996).

[2] P. E. Blöchl, *Projector Augmented-Wave Method*, Phys. Rev. B **50**, 17953 (1994).

[3] J. P. Perdew, K. Burke, and M. Ernzerhof, *Generalized Gradient Approximation Made Simple*, Phys. Rev. Lett. **77**, 3865 (1996).

[4] J. P. Perdew, J. A. Chevary, S. H. Vosko, K. A. Jackson, M. R. Pederson, D. J. Singh, and C. Fiolhais, *Atoms, Molecules, Solids, and Surfaces: Applications of the Generalized Gradient Approximation for Exchange and Correlation*, Phys. Rev. B **46**, 6671 (1992).

[5] Z. Lu, Z. W. Chen, and C. V. Singh, *Neural Network-Assisted Development of High-Entropy Alloy Catalysts: Decoupling Ligand and Coordination Effects*, Matter **3**, 1318 (2020).

[6] L. T. Roling and F. Abild-Pedersen, *Structure-Sensitive Scaling Relations: Adsorption Energies from Surface Site Stability*, ChemCatChem **10**, 1643 (2018).

[7] M. Andersen, S. V. Levchenko, M. Scheffler, and K. Reuter, *Beyond Scaling Relations for the Description of Catalytic Materials*, ACS Catal. **9**, 2752 (2019).

[8] M. J. Hoffmann, A. J. Medford, and T. Bligaard, *Framework for Scalable Adsorbate–Adsorbate Interaction Models*, J. Phys. Chem. C **120**, 13087 (2016).

[9] S. Ghosh, S. Hariharan, and A. K. Tiwari, *Water Adsorption and Dissociation on Copper/Nickel Bimetallic Surface Alloys: Effect of Surface Temperature on Reactivity*, J. Phys. Chem. C **121**, 16351 (2017).

[10] L.-Y. Gan, R.-Y. Tian, X.-B. Yang, H.-D. Lu, and Y.-J. Zhao, *Catalytic Reactivity of CuNi Alloys toward $H_2O$ and CO Dissociation for an Efficient Water–Gas Shift: A DFT Study*, J. Phys. Chem. C **116**, 745 (2012).

[11] H. Xin, A. Holewinski, N. Schweitzer, E. Nikolla, and S. Linic, *Electronic Structure Engineering in Heterogeneous Catalysis: Identifying Novel Alloy Catalysts Based on Rapid Screening for Materials with Desired Electronic Properties*, Top. Catal. **55**, 376 (2012).

[12] F. Calle-Vallejo, J. I. Martínez, J. M. García-Lastra, J. Rossmeisl, and M. T. M. Koper, *Physical and Chemical Nature of the Scaling Relations between Adsorption Energies of Atoms on Metal Surfaces*, Phys. Rev. Lett. **108**, 116103 (2012).

[13] H. Xin, A. Holewinski, and S. Linic, *Predictive Structure–Reactivity Models for Rapid Screening of Pt-Based Multimetallic Electrocatalysts for the Oxygen Reduction Reaction*, ACS Catal. **2**, 12 (2012).

[14] X. Ma, Z. Li, L. E. K. Achenie, and H. Xin, *Machine-Learning-Augmented Chemisorption Model for $CO_2$ Electroreduction Catalyst Screening*, J. Phys. Chem. Lett. **6**, 3528 (2015).

[15] O. Mamun, K. T. Winther, J. R. Boes, and T. Bligaard, *High-Throughput Calculations of Catalytic Properties of Bimetallic Alloy Surfaces*, Sci. Data **6**, 76 (2019).

[16] E. J. Evans, H. Li, W. Y. Yu, G. M. Mullen, G. Henkelman, and C. B. Mullins, *Mechanistic Insights on Ethanol Dehydrogenation on Pd-Au Model Catalysts: A Combined Experimental and DFT Study*, Phys. Chem. Chem. Phys. **19**, 30578 (2017).

[17] S. Wang, B. Temel, J. Shen, G. Jones, L. C. Grabow, F. Studt, T. Bligaard, F. Abild-Pedersen, C. H. Christensen, and J. K. Nørskov, *Universal Brønsted-Evans-Polanyi Relations for C–C, C–O, C–N, N–O, N–N, and O–O Dissociation Reactions*, Catal. Letters **141**, 370 (2011).

[18] B. Hammer, L. B. Hansen, and J. K. Nørskov, *Improved Adsorption Energetics within Density-Functional Theory Using Revised Perdew-Burke-Ernzerhof Functionals*, Phys. Rev. B **59**, 7413 (1999).

[19] J. Wellendorff, K. T. Lundgaard, A. Møgelhøj, V. Petzold, D. D. Landis, J. K. Nørskov, T. Bligaard, and K. W. Jacobsen, *Density Functionals for Surface Science: Exchange-Correlation Model Development with Bayesian Error Estimation*, Phys. Rev. B **85**, 235149 (2012).

[20] S. Grimme, J. Antony, S. Ehrlich, and H. Krieg, *A Consistent and Accurate Ab Initio Parametrization of Density Functional Dispersion Correction (DFT-D) for the 94 Elements H-Pu*, J. Chem. Phys. **132**, 154104 (2010).

[21] E. Hansen and M. Neurock, *Predicting Lateral Surface Interactions through Density Functional Theory: Application to Oxygen on Rh(100)*, Surf. Sci. **441**, 410 (1999).

[22] N. İnoğlu and J. R. Kitchin, *Simple Model Explaining and Predicting Coverage-Dependent Atomic Adsorption Energies on Transition Metal Surfaces*, Phys. Rev. B **82**, 045414 (2010).

[23] L. C. Grabow, B. Hvolbæk, and J. K. Nørskov, *Understanding Trends in Catalytic Activity: The Effect of Adsorbate–Adsorbate Interactions for CO Oxidation over Transition Metals*, Top. Catal. **53**, 298 (2010).

[24] C. Stampfl, H. J. Kreuzer, S. H. Payne, H. Pfnür, and M. Scheffler, *First-Principles Theory of Surface Thermodynamics and Kinetics*, Phys. Rev. Lett. **83**, 2993 (1999).

[25] R. Drautz, R. Singer, and M. Fähnle, *Cluster Expansion Technique: An Efficient Tool to Search for Ground-State Configurations of Adatoms on Plane Surfaces*, Phys. Rev. B **67**, 035418 (2003).

[26] C. Wu, D. J. Schmidt, C. Wolverton, and W. F. Schneider, *Accurate Coverage-Dependence Incorporated into First-Principles Kinetic Models: Catalytic NO Oxidation on Pt (111)*, J. Catal. **286**, 88 (2012).

[27] W. Gao, Y. Chen, B. Li, S.-P. Liu, X. Liu, and Q. Jiang, *Determining the Adsorption Energies of Small Molecules with the Intrinsic Properties of Adsorbates and Substrates*, Nat. Commun. **11**, 1196 (2020).

[28] J. K. Nørskov and N. D. Lang, *Effective-Medium Theory of Chemical Binding: Application to Chemisorption*, Phys. Rev. B **21**, 2131 (1980).

[29] F. Abild-Pedersen, J. Greeley, F. Studt, J. Rossmeisl, T. R. Munter, P. G. Moses, E. Skúlason, T. Bligaard, and J. K. Nørskov, *Scaling Properties of Adsorption Energies for Hydrogen-Containing Molecules on Transition-Metal Surfaces*, Phys. Rev. Lett. **99**, 016105 (2007).

[30] S. Trasatti, *Work Function, Electronegativity, and Electrochemical Behaviour of Metals*, J. Electroanal. Chem. Interfacial Electrochem. **39**, 163 (1972).

[31] S. Wu, Y. Pan, J. Lu, N. Wang, W. Dai, and T. Lu, *Effect of the Addition of Mg, Ti, Ni on the Decoloration Performance of AlCrFeMn High Entropy Alloy*, J. Mater. Sci. Technol. **35**, 1629 (2019).

[32] H.-J. Qiu, G. Fang, J. Gao, Y. Wen, J. Lv, H. Li, G. Xie, X. Liu, and S. Sun, *Noble Metal-Free Nanoporous High-Entropy Alloys as Highly Efficient Electrocatalysts for Oxygen Evolution Reaction*, ACS Mater. Lett. **1**, 526 (2019).

[33] P. Xie, Y. Yao, Z. Huang, Z. Liu, J. Zhang, T. Li, G. Wang, R. Shahbazian-Yassar, L. Hu, and C. Wang, *Highly Efficient Decomposition of Ammonia Using High-Entropy Alloy Catalysts*, Nat. Commun. **10**, 4011 (2019).

[34] T. Löffler, H. Meyer, A. Savan, P. Wilde, A. Garzón Manjón, Y.-T. Chen, E. Ventosa, C. Scheu, A. Ludwig, and W. Schuhmann, *Discovery of a Multinary Noble Metal-Free Oxygen Reduction Catalyst*, Adv. Energy Mater. **8**, 1802269 (2018).

[35] E. L. Clark, C. Hahn, T. F. Jaramillo, and A. T. Bell, *Electrochemical $CO_2$ Reduction over Compressively Strained CuAg Surface Alloys with Enhanced Multi-Carbon Oxygenate Selectivity*, J. Am. Chem. Soc. **139**, 15848 (2017).

[36] V. Tripkovic, H. A. Hansen, J. Rossmeisl, and T. Vegge, *First Principles Investigation of the Activity of Thin Film Pt, Pd and Au Surface Alloys for Oxygen Reduction*, Phys. Chem. Chem. Phys. **17**, 11647 (2015).

[37] K. P. Kuhl, T. Hatsukade, E. R. Cave, D. N. Abram, J. Kibsgaard, and T. F. Jaramillo, *Electrocatalytic Conversion of Carbon Dioxide to Methane and Methanol on Transition Metal Surfaces*, J. Am. Chem. Soc. **136**, 14107 (2014).

[38] J. K. Nørskov, T. Bligaard, A. Logadottir, J. R. Kitchin, J. G. Chen, S. Pandelov, and U. Stimming, *Trends in the Exchange Current for Hydrogen Evolution*, J. Electrochem. Soc. **152**, J23 (2005).

[39] M. Escudero-Escribano, P. Malacrida, M. H. Hansen, U. G. Vej-Hansen, A. Velazquez-Palenzuela, V. Tripkovic, J. Schiotz, J. Rossmeisl, I. E. L. Stephens, and I. Chorkendorff, *Tuning the Activity of Pt Alloy Electrocatalysts by Means of the Lanthanide Contraction*, Science **352**, 73 (2016).

[40] T. Bligaard, J. K. Nørskov, S. Dahl, J. Matthiesen, C. H. Christensen, and J. Sehested, *The Brønsted–Evans–Polanyi Relation and the Volcano Curve in Heterogeneous Catalysis*, J. Catal. **224**, 206 (2004).

[41] J. K. Pedersen, T. A. A. Batchelor, D. Yan, L. E. J. Skjegstad, and J. Rossmeisl, *Surface Electrocatalysis on High-Entropy Alloys*, Curr. Opin. Electrochem. **26**, 100651 (2021).

[42] G. Zhang, *Understanding the Role of van Der Waals Forces in Solids from First Principles*, Freie Universität Berlin (2014).

[43] X. Guan, C. Zhao, X. Liu, S. Liu, W. Gao, and Q. Jiang, *Universal Principle to Describe Reactivity and Selectivity of $CO_2$ Electroreduction on Transition Metals and Single-Atom Catalysts*, J. Phys. Chem. C **124**, 25898 (2020).

[44] L. Qi, W. Gao, and Q. Jiang, *Effective Descriptor for Designing High-Performance Catalysts for the Hydrogen Evolution Reaction*, J. Phys. Chem. C **124**, 23134 (2020).
